# Supplementary material for: SMEFT ATLAS of $\Delta F=2$ Transitions
Source: arXiv:2009.07276 ancillary file (2020-09-15)
Supplement: Supplementary file 1 [file ABBKsup.pdf]

# Supplementary Material

# SMEFT ATLAS of $\Delta F = 2$ Transitions

**Jason Aebischer**[a], **Christoph Bobeth**[b], **Andrzej J. Buras**[c] **and Jacky Kumar**[d]

[a]Department of Physics, University of California at San Diego, La Jolla, CA 92093, USA

[b]Physik Department T31, James-Franck-Straße 1, Technische Universität München, D–85748 Garching, Germany

[c]TUM Institute for Advanced Study, Lichtenbergstr. 2a, D–85747 Garching, Germany

[d]Physique des Particules, Universite de Montreal, C.P. 6128, succ. centre-ville, Montreal, QC, Canada H3C 3J7

# Tables for $P_a^{ij}(\Lambda)$ Coefficients at 5TeV

In the following tables the magnitude and argument of the $P_a^{ij}(\Lambda)$ coefficients entering in the SMEFT master formulae Eq. (23) for $[\mathcal{M}_{12}^{ij}]_{\rm BSM}$ are shown for the $B_s$, $B_d$, $K^0$ and $D^0$ meson systems in the Warsaw-down and up bases. Note that entries are set to zero for four-quark operators when they are below $10^{-3}$ and for semileptonic operators below $10^{-4}$. Further, we skip rows if all entries for an operator for a given flavour index are zero. Similarly, tables are not shown if all the entries are zero.

| $[\mathcal{C}_{qq}^{(1)}]_{ijkl}$(Warsaw-down) | | | | | | | | |
|---|---|---|---|---|---|---|---|---|
| $ijkl$ | $\lvert P_a^{sb}\rvert$ | $\arg(P_a^{sb})$ | $\lvert P_a^{db}\rvert$ | $\arg(P_a^{db})$ | $\lvert P_a^{sd}\rvert$ | $\arg(P_a^{sd})$ | $\lvert P_a^{cu}\rvert$ | $\arg(P_a^{cu})$ |
| 1111 | - | - | $(6.08)10^{-3}$ | -136 | - | - | $(2.35)10^{5}$ | -180 |
| 1112 | - | - | 0.03 | 21 | 6.35 | 23 | $(9.69)10^{5}$ | 0 |
| 1113 | - | - | 39.17 | -158 | 0.01 | 24 | $(4.54)10^{4}$ | -1 |
| 1122 | - | - | - | - | - | - | $(2.35)10^{5}$ | 0 |
| 1123 | $(2.68)10^{-3}$ | -1 | - | - | $(1.40)10^{-3}$ | -135 | $(1.22)10^{4}$ | 18 |
| 1133 | - | - | $(8.79)10^{-3}$ | 44 | - | - | 174.98 | 73 |
| 1212 | - | - | 0.14 | 178 | $(8.87)10^{5}$ | -180 | $(4.46)10^{6}$ | 180 |
| 1213 | - | - | 179.76 | -1 | $(1.50)10^{3}$ | -179 | $(1.98)10^{5}$ | -180 |
| 1221 | - | - | - | - | - | - | $(2.35)10^{5}$ | 0 |
| 1222 | $(1.26)10^{-3}$ | 21 | $(1.62)10^{-3}$ | -159 | 14.23 | -157 | $(9.69)10^{5}$ | 180 |
| 1223 | $(1.25)10^{-3}$ | 156 | 0.14 | 22 | 0.13 | -156 | $(4.54)10^{4}$ | 179 |
| 1231 | 0.03 | 179 | $(5.44)10^{-3}$ | 45 | 0.02 | 45 | $(1.22)10^{4}$ | 18 |
| 1232 | 1.70 | -158 | - | - | 330.14 | 22 | $(1.64)10^{4}$ | -99 |
| 1233 | $(1.73)10^{-3}$ | -159 | 0.04 | -159 | 3.05 | 23 | 719.75 | -107 |
| 1313 | - | - | $(2.27)10^{5}$ | -180 | 2.56 | -178 | $(8.86)10^{3}$ | -180 |
| 1322 | - | - | 0.04 | -158 | 0.03 | -156 | $(4.54)10^{4}$ | 179 |
| 1323 | 0.10 | -23 | 2.97 | -157 | - | - | $(2.05)10^{3}$ | 180 |
| 1331 | - | - | 0.13 | -136 | - | - | 174.98 | 73 |
| 1332 | 0.03 | 21 | 0.58 | 21 | 0.65 | 23 | 719.74 | -107 |
| 1333 | - | - | 68.10 | 22 | $(7.55)10^{-3}$ | 24 | 33.76 | -108 |
| 2222 | $(5.47)10^{-3}$ | 178 | - | - | - | - | $(2.35)10^{5}$ | 180 |
| 2223 | 7.73 | -1 | - | - | $(5.24)10^{-3}$ | 44 | $(1.22)10^{4}$ | -162 |
| 2233 | $(7.91)10^{-3}$ | -2 | - | - | - | - | 174.94 | -107 |
| 2323 | $(9.80)10^{3}$ | 180 | - | - | 0.12 | -136 | 417.93 | -175 |
| 2332 | 0.11 | 178 | - | - | - | - | 174.94 | -107 |
| 2333 | 13.61 | 179 | - | - | $(1.65)10^{-3}$ | -135 | 9.11 | -90 |
| 3333 | 0.01 | 178 | 0.02 | -136 | - | - | 0.13 | -34 |

Table 1: The modulus (in the units of $\text{TeV}^2$) and the argument (in degrees) of $P_a^{ij}(\Lambda)$ in Warsaw-down basis for meson systems at scale $\Lambda = 5\,\text{TeV}$ is shown.

| $[\mathcal{C}_{qq}^{(1)}]_{ijkl}$ **(Warsaw-up)** | | | | | | | | |
|---|---|---|---|---|---|---|---|---|
| $ijkl$ | $\lvert P_a^{sb}\rvert$ | $\arg(P_a^{sb})$ | $\lvert P_a^{db}\rvert$ | $\arg(P_a^{db})$ | $\lvert P_a^{sd}\rvert$ | $\arg(P_a^{sd})$ | $\lvert P_a^{cu}\rvert$ | $\arg(P_a^{cu})$ |
| 1111 | $(6.22)10^{-3}$ | 35 | 2.72 | 34 | $(4.23)10^{4}$ | -180 | - | - |
| 1112 | 0.08 | 90 | 31.59 | 108 | $(1.74)10^{5}$ | -180 | 57.49 | 23 |
| 1113 | 1.75 | 107 | 766.68 | 107 | $(7.14)10^{3}$ | 0 | 0.07 | 23 |
| 1122 | 0.31 | 107 | 7.31 | -73 | $(4.23)10^{4}$ | -0 | - | - |
| 1123 | 7.58 | 107 | 176.08 | -73 | $(3.31)10^{3}$ | -169 | $(6.31)10^{-3}$ | 96 |
| 1133 | 0.31 | -74 | 6.90 | 129 | 67.48 | 23 | - | - |
| 1212 | 0.75 | 175 | 370.34 | 180 | $(8.01)10^{5}$ | -180 | $(4.94)10^{6}$ | 180 |
| 1213 | 20.41 | -180 | $(8.93)10^{3}$ | -180 | $(3.26)10^{4}$ | 1 | $(6.28)10^{3}$ | 180 |
| 1221 | 0.32 | 107 | 7.31 | -73 | $(4.23)10^{4}$ | -0 | - | - |
| 1222 | 4.28 | 162 | 84.73 | 1 | $(1.74)10^{5}$ | -0 | 57.05 | -158 |
| 1223 | 88.58 | -180 | $(2.05)10^{3}$ | -0 | $(7.13)10^{3}$ | 180 | 0.08 | -159 |
| 1231 | 7.59 | 107 | 176.08 | -73 | $(3.31)10^{3}$ | -169 | $(6.25)10^{-3}$ | 96 |
| 1232 | 32.94 | 107 | 40.43 | 112 | $(6.76)10^{3}$ | -157 | 537.35 | -107 |
| 1233 | 4.24 | -19 | 79.97 | -157 | 277.42 | 23 | 0.68 | -107 |
| 1313 | 492.43 | -180 | $(2.15)10^{5}$ | -180 | $(1.32)10^{3}$ | -178 | 7.99 | 180 |
| 1322 | 88.57 | -180 | $(2.05)10^{3}$ | -0 | $(7.13)10^{3}$ | 180 | 0.07 | -157 |
| 1323 | $(2.13)10^{3}$ | -180 | $(4.96)10^{4}$ | -0 | 294.33 | 0 | - | - |
| 1331 | 0.31 | -74 | 6.84 | 129 | 66.95 | 23 | - | - |
| 1332 | 4.21 | -19 | 79.35 | -157 | 275.26 | 23 | 0.68 | -107 |
| 1333 | 87.80 | -1 | $(1.94)10^{3}$ | -158 | 11.38 | -157 | - | - |
| 2222 | 15.94 | -180 | 19.60 | 180 | $(4.22)10^{4}$ | 180 | - | - |
| 2223 | 383.96 | -180 | 472.25 | 180 | $(3.30)10^{3}$ | 11 | $(6.17)10^{-3}$ | -85 |
| 2233 | 15.80 | -1 | 18.50 | 22 | 67.38 | -157 | - | - |
| 2323 | $(9.28)10^{3}$ | -180 | $(1.14)10^{4}$ | 180 | 125.17 | -158 | 0.06 | -34 |
| 2332 | 15.68 | -1 | 18.36 | 22 | 66.85 | -157 | - | - |
| 2333 | 380.57 | -1 | 445.71 | 22 | 5.27 | 34 | - | - |
| 3333 | 15.66 | 178 | 17.46 | -136 | 0.11 | -134 | - | - |

Table 2: The modulus (in the units of $\text{TeV}^2$) and the argument (in degrees) of $P_a^{ij}(\Lambda)$ in Warsaw-up basis for meson systems at scale $\Lambda = 5\,\text{TeV}$ is shown.

| $\left[\mathcal{C}_{qq}^{(3)}\right]_{ijkl}$**(Warsaw-down)** | | | | | | | | |
|---|---|---|---|---|---|---|---|---|
| $ijkl$ | $\lvert P_a^{sb}\rvert$ | $\arg(P_a^{sb})$ | $\lvert P_a^{db}\rvert$ | $\arg(P_a^{db})$ | $\lvert P_a^{sd}\rvert$ | $\arg(P_a^{sd})$ | $\lvert P_a^{cu}\rvert$ | $\arg(P_a^{cu})$ |
| 1111 | - | - | $(2.03)10^{-3}$ | -136 | - | - | $(2.35)10^{5}$ | -180 |
| 1112 | - | - | 0.02 | 21 | 6.24 | 23 | $(9.69)10^{5}$ | 0 |
| 1113 | - | - | 38.19 | -158 | 0.01 | 24 | $(4.54)10^{4}$ | -1 |
| 1122 | $(2.06)10^{-3}$ | -2 | $(2.32)10^{-3}$ | 44 | $(1.69)10^{-3}$ | -134 | $(2.35)10^{5}$ | 0 |
| 1123 | 0.16 | 179 | $(9.39)10^{-3}$ | 45 | 0.04 | 45 | $(1.22)10^{4}$ | 18 |
| 1133 | $(1.70)10^{-3}$ | -2 | 0.23 | -136 | - | - | 174.98 | 73 |
| 1212 | - | - | 0.14 | 178 | $(8.87)10^{5}$ | -180 | $(4.46)10^{6}$ | 180 |
| 1213 | - | - | 179.76 | -1 | $(1.50)10^{3}$ | -179 | $(1.98)10^{5}$ | -180 |
| 1221 | - | - | - | - | - | - | $(2.35)10^{5}$ | 0 |
| 1222 | - | - | 0.01 | -159 | 14.29 | -157 | $(9.69)10^{5}$ | 180 |
| 1223 | - | - | 0.03 | -158 | 0.03 | 23 | $(4.54)10^{4}$ | 179 |
| 1231 | $(3.06)10^{-3}$ | 179 | $(4.61)10^{-3}$ | -136 | 0.01 | -135 | $(1.22)10^{4}$ | 18 |
| 1232 | 1.70 | -158 | $(2.56)10^{-3}$ | 20 | 330.12 | 22 | $(1.64)10^{4}$ | -99 |
| 1233 | 0.05 | 21 | 1.06 | 21 | 0.72 | -157 | 719.77 | -107 |
| 1313 | - | - | $(2.27)10^{5}$ | -180 | 2.56 | -178 | $(8.86)10^{3}$ | -180 |
| 1322 | $(2.05)10^{-3}$ | 154 | 0.83 | 22 | 0.22 | -156 | $(4.54)10^{4}$ | 179 |
| 1323 | 0.11 | -23 | 2.82 | -157 | - | - | $(2.05)10^{3}$ | 180 |
| 1331 | - | - | 0.10 | 44 | - | - | 174.98 | 73 |
| 1332 | 0.02 | -159 | 0.44 | -159 | 5.13 | 23 | 719.81 | -107 |
| 1333 | - | - | 70.58 | 20 | 0.02 | 24 | 33.71 | -108 |
| 2222 | $(1.79)10^{-3}$ | 178 | - | - | - | - | $(2.35)10^{5}$ | 180 |
| 2223 | 7.60 | -1 | - | - | $(4.95)10^{-3}$ | 44 | $(1.22)10^{4}$ | -162 |
| 2233 | 0.21 | 178 | $(1.94)10^{-3}$ | 44 | - | - | 174.94 | -107 |
| 2323 | $(9.80)10^{3}$ | 180 | - | - | 0.12 | -136 | 417.90 | -175 |
| 2332 | 0.09 | -2 | - | - | - | - | 174.95 | -107 |
| 2333 | 12.81 | 179 | $(1.56)10^{-3}$ | -137 | $(4.33)10^{-3}$ | -135 | 9.09 | -89 |
| 3333 | 0.02 | -2 | 0.02 | 44 | - | - | 0.13 | -34 |

Table 3: The modulus (in the units of $\mathrm{TeV}^2$) and the argument (in degrees) of $P_a^{ij}(\Lambda)$ in Warsaw-down basis for meson systems at scale $\Lambda = 5\,\mathrm{TeV}$ is shown.

| $[\mathcal{C}_{qq}^{(3)}]_{ijkl}$ **(Warsaw-up)** | | | | | | | | |
|---|---|---|---|---|---|---|---|---|
| $ijkl$ | $\|P_a^{sb}\|$ | $\arg(P_a^{sb})$ | $\|P_a^{db}\|$ | $\arg(P_a^{db})$ | $\|P_a^{sd}\|$ | $\arg(P_a^{sd})$ | $\|P_a^{cu}\|$ | $\arg(P_a^{cu})$ |
| 1111 | $(6.22)10^{-3}$ | 36 | 2.73 | 34 | $(4.23)10^{4}$ | -180 | - | - |
| 1112 | 0.08 | 90 | 31.59 | 108 | $(1.74)10^{5}$ | -180 | 57.29 | 23 |
| 1113 | 1.76 | 108 | 766.65 | 107 | $(7.14)10^{3}$ | 0 | 0.07 | 23 |
| 1122 | 0.32 | 108 | 7.31 | -73 | $(4.23)10^{4}$ | -0 | - | - |
| 1123 | 7.64 | 108 | 176.09 | -73 | $(3.31)10^{3}$ | -169 | $(6.10)10^{-3}$ | 96 |
| 1133 | 0.31 | -72 | 6.81 | 129 | 66.66 | 23 | - | - |
| 1212 | 0.75 | 175 | 370.34 | 180 | $(8.01)10^{5}$ | -180 | $(4.94)10^{6}$ | 180 |
| 1213 | 20.41 | -180 | $(8.93)10^{3}$ | -180 | $(3.26)10^{4}$ | 1 | $(6.28)10^{3}$ | 180 |
| 1221 | 0.31 | 107 | 7.31 | -73 | $(4.23)10^{4}$ | -0 | - | - |
| 1222 | 4.28 | 162 | 84.75 | 1 | $(1.74)10^{5}$ | -0 | 56.85 | -158 |
| 1223 | 88.58 | -180 | $(2.05)10^{3}$ | -0 | $(7.13)10^{3}$ | 180 | 0.06 | -155 |
| 1231 | 7.59 | 107 | 176.08 | -73 | $(3.31)10^{3}$ | -169 | $(6.29)10^{-3}$ | 96 |
| 1232 | 32.94 | 107 | 40.43 | 112 | $(6.76)10^{3}$ | -157 | 537.35 | -107 |
| 1233 | 4.19 | -19 | 78.99 | -157 | 274.02 | 23 | 0.68 | -107 |
| 1313 | 492.43 | -180 | $(2.15)10^{5}$ | -180 | $(1.32)10^{3}$ | -178 | 7.99 | 180 |
| 1322 | 88.61 | -180 | $(2.05)10^{3}$ | -0 | $(7.13)10^{3}$ | 180 | 0.07 | -158 |
| 1323 | $(2.13)10^{3}$ | -180 | $(4.96)10^{4}$ | -0 | 294.34 | 0 | - | - |
| 1331 | 0.31 | -74 | 6.94 | 129 | 67.94 | 23 | - | - |
| 1332 | 4.27 | -19 | 80.51 | -157 | 279.30 | 23 | 0.68 | -107 |
| 1333 | 87.94 | -1 | $(1.93)10^{3}$ | -158 | 11.37 | -157 | - | - |
| 2222 | 15.95 | -180 | 19.61 | 180 | $(4.22)10^{4}$ | 180 | - | - |
| 2223 | 384.08 | -180 | 472.38 | 180 | $(3.30)10^{3}$ | 11 | $(6.35)10^{-3}$ | -85 |
| 2233 | 15.61 | -1 | 18.28 | 22 | 66.55 | -157 | - | - |
| 2323 | $(9.28)10^{3}$ | -180 | $(1.14)10^{4}$ | 180 | 125.19 | -158 | 0.06 | -34 |
| 2332 | 15.90 | -1 | 18.62 | 22 | 67.83 | -157 | - | - |
| 2333 | 381.34 | -1 | 446.60 | 22 | 5.29 | 34 | - | - |
| 3333 | 15.67 | 178 | 17.47 | -136 | 0.11 | -134 | - | - |

Table 4: The modulus (in the units of $\text{TeV}^2$) and the argument (in degrees) of $P_a^{ij}(\Lambda)$ in Warsaw-up basis for meson systems at scale $\Lambda = 5\,\text{TeV}$ is shown.

| $[\mathcal{C}_{qd}^{(1)}]_{ijkl}$**(Warsaw-down)** | | | | | | | | |
|---|---|---|---|---|---|---|---|---|
| $ijkl$ | $\lvert P_a^{sb}\rvert$ | $\arg(P_a^{sb})$ | $\lvert P_a^{db}\rvert$ | $\arg(P_a^{db})$ | $\lvert P_a^{sd}\rvert$ | $\arg(P_a^{sd})$ | $\lvert P_a^{cu}\rvert$ | $\arg(P_a^{cu})$ |
| 1111 | - | - | - | - | $(1.07)10^{-3}$ | 45 | - | - |
| 1112 | - | - | 0.01 | -159 | 846.53 | -154 | - | - |
| 1113 | - | - | 244.62 | 22 | 0.05 | -156 | - | - |
| 1122 | - | - | - | - | $(1.07)10^{-3}$ | -135 | - | - |
| 1123 | $(8.29)10^{-3}$ | 179 | - | - | - | - | $(1.47)10^{-3}$ | 18 |
| 1133 | - | - | - | - | - | - | $(1.05)10^{-3}$ | 73 |
| 1211 | - | - | - | - | 63.27 | -114 | - | - |
| 1212 | - | - | 0.05 | -2 | $(1.31)10^{8}$ | 0 | - | - |
| 1213 | - | - | $(1.11)10^{3}$ | 179 | $(6.44)10^{3}$ | 1 | $(1.16)10^{-3}$ | -180 |
| 1221 | - | - | - | - | 0.12 | 46 | - | - |
| 1222 | - | - | - | - | 63.26 | 66 | $(2.31)10^{-3}$ | 180 |
| 1223 | $(6.93)10^{-3}$ | -24 | $(1.27)10^{-3}$ | -158 | $(7.32)10^{-3}$ | 24 | $(5.44)10^{-3}$ | 179 |
| 1231 | - | - | 0.03 | -135 | - | - | - | - |
| 1232 | 10.00 | 22 | - | - | 69.20 | -158 | $(1.97)10^{-3}$ | -99 |
| 1233 | - | - | - | - | $(3.10)10^{-3}$ | -157 | $(4.33)10^{-3}$ | -107 |
| 1311 | - | - | 0.76 | 21 | 0.25 | -156 | - | - |
| 1312 | - | - | 69.15 | 179 | $(2.23)10^{5}$ | 1 | - | - |
| 1313 | - | - | $(1.41)10^{6}$ | 0 | 10.95 | 2 | - | - |
| 1321 | - | - | - | - | 2.81 | -135 | - | - |
| 1322 | - | - | $(1.65)10^{-3}$ | -158 | 0.25 | 24 | - | - |
| 1323 | 0.57 | 157 | 1.61 | 23 | - | - | - | - |
| 1331 | - | - | 0.74 | 44 | - | - | - | - |
| 1332 | 0.14 | -159 | - | - | 0.12 | -157 | - | - |
| 1333 | - | - | 0.78 | -159 | - | - | - | - |
| 2211 | - | - | - | - | $(2.40)10^{-3}$ | -135 | - | - |
| 2212 | - | - | - | - | $(2.01)10^{3}$ | 24 | - | - |
| 2213 | - | - | 0.18 | 22 | 0.11 | 23 | - | - |
| 2222 | $(2.23)10^{-3}$ | -2 | - | - | $(2.40)10^{-3}$ | 45 | - | - |
| 2223 | 45.64 | 179 | - | - | $(1.11)10^{-3}$ | -136 | $(1.47)10^{-3}$ | -162 |
| 2233 | $(2.23)10^{-3}$ | 178 | - | - | - | - | $(1.05)10^{-3}$ | -107 |
| 2311 | - | - | - | - | 0.06 | 44 | - | - |
| 2312 | - | - | - | - | 18.00 | 24 | - | - |
| 2313 | 0.07 | 158 | 18.89 | 23 | - | - | - | - |
| 2321 | 0.03 | 22 | - | - | $(4.90)10^{4}$ | -158 | - | - |
| 2322 | 2.81 | 179 | - | - | 0.06 | -136 | - | - |
| 2323 | $(5.77)10^{4}$ | -0 | - | - | 0.03 | 44 | - | - |
| 2331 | - | - | 3.37 | -159 | 2.40 | -157 | - | - |
| 2332 | 0.63 | -2 | - | - | - | - | - | - |
| 2333 | 2.80 | -1 | - | - | - | - | - | - |
| 3312 | - | - | 0.02 | 21 | 421.07 | -157 | - | - |
| 3313 | - | - | 437.23 | -158 | 0.02 | -156 | - | - |
| 3322 | $(3.99)10^{-3}$ | 178 | - | - | - | - | - | - |
| 3323 | 81.49 | -1 | - | - | - | - | - | - |
| 3333 | $(3.98)10^{-3}$ | -2 | - | - | - | - | - | - |

Table 5: The modulus (in the units of $\mathrm{TeV}^2$) and the argument (in degrees) of $P_a^{ij}(\Lambda)$ in Warsaw-down basis for meson systems at scale $\Lambda = 5\,\mathrm{TeV}$ is shown.

| $[\mathcal{C}_{qd}^{(1)}]_{ijkl}$**(Warsaw-up)** | | | | | | | | |
|---|---|---|---|---|---|---|---|---|
| $ijkl$ | $\lvert P_a^{sb}\rvert$ | $\arg(P_a^{sb})$ | $\lvert P_a^{db}\rvert$ | $\arg(P_a^{db})$ | $\lvert P_a^{sd}\rvert$ | $\arg(P_a^{sd})$ | $\lvert P_a^{cu}\rvert$ | $\arg(P_a^{cu})$ |
| 1111 | - | - | $(2.56)10^{-3}$ | -51 | 27.85 | -153 | - | - |
| 1112 | - | - | 0.24 | 106 | $(2.87)10^{7}$ | 0 | - | - |
| 1113 | - | - | $(4.89)10^{3}$ | -73 | $(1.40)10^{3}$ | 1 | - | - |
| 1122 | $(2.24)10^{-3}$ | 106 | - | - | 27.85 | 27 | - | - |
| 1123 | 45.97 | -73 | $(5.67)10^{-3}$ | -43 | 15.13 | -158 | - | - |
| 1133 | $(2.25)10^{-3}$ | -74 | $(2.57)10^{-3}$ | 129 | - | - | - | - |
| 1211 | - | - | 0.03 | 23 | 61.74 | -123 | - | - |
| 1212 | - | - | 2.79 | 179 | $(1.25)10^{8}$ | 0 | - | - |
| 1213 | $(1.33)10^{-3}$ | -93 | $(5.70)10^{4}$ | 0 | $(6.11)10^{3}$ | 1 | $(1.23)10^{-3}$ | 180 |
| 1221 | - | - | 0.06 | -74 | $(6.62)10^{6}$ | 180 | - | - |
| 1222 | 0.03 | 161 | - | - | 61.74 | 57 | $(2.57)10^{-3}$ | 180 |
| 1223 | 536.07 | 0 | 0.06 | 21 | 3.49 | 22 | $(5.77)10^{-3}$ | 180 |
| 1231 | $(1.43)10^{-3}$ | -69 | $(1.12)10^{3}$ | 107 | 324.02 | -179 | - | - |
| 1232 | 199.58 | -73 | - | - | 65.64 | -158 | $(2.15)10^{-3}$ | -107 |
| 1233 | 0.03 | -19 | 0.03 | -157 | $(2.79)10^{-3}$ | -157 | $(4.82)10^{-3}$ | -107 |
| 1311 | - | - | 0.74 | 21 | 5.64 | 22 | - | - |
| 1312 | - | - | 67.33 | 179 | $(5.09)10^{6}$ | -179 | - | - |
| 1313 | 0.02 | 153 | $(1.37)10^{6}$ | 0 | 249.25 | -178 | - | - |
| 1321 | $(6.79)10^{-3}$ | 22 | $(2.13)10^{-3}$ | 128 | $(2.57)10^{5}$ | 22 | - | - |
| 1322 | 0.63 | 179 | $(1.61)10^{-3}$ | -158 | 5.67 | -158 | - | - |
| 1323 | $(1.29)10^{4}$ | 0 | 1.56 | 23 | 0.14 | -136 | - | - |
| 1331 | $(2.05)10^{-3}$ | 106 | 43.64 | -51 | 12.58 | 23 | - | - |
| 1332 | 8.13 | 106 | $(2.31)10^{-3}$ | 128 | 2.66 | 23 | - | - |
| 1333 | 0.63 | -1 | 0.75 | -159 | - | - | - | - |
| 2211 | - | - | $(6.87)10^{-3}$ | -158 | 37.66 | 20 | - | - |
| 2212 | $(1.25)10^{-3}$ | 21 | 0.64 | -1 | $(2.87)10^{7}$ | 180 | - | - |
| 2213 | 0.08 | 1 | $(1.31)10^{4}$ | 180 | $(1.40)10^{3}$ | -179 | - | - |
| 2222 | 0.11 | 179 | - | - | 37.66 | -160 | - | - |
| 2223 | $(2.32)10^{3}$ | 0 | 0.02 | -163 | 15.10 | 22 | - | - |
| 2233 | 0.11 | -1 | $(6.90)10^{-3}$ | 22 | - | - | - | - |
| 2311 | - | - | 0.16 | -158 | 2.53 | -146 | - | - |
| 2312 | - | - | 15.49 | -1 | $(1.17)10^{6}$ | 1 | - | - |
| 2313 | 0.13 | 169 | $(3.16)10^{5}$ | 180 | 57.33 | 2 | - | - |
| 2321 | 0.03 | 22 | 0.02 | -159 | $(1.11)10^{6}$ | 22 | - | - |
| 2322 | 2.73 | 179 | - | - | 2.53 | 34 | - | - |
| 2323 | $(5.61)10^{4}$ | 0 | 0.36 | -157 | 0.59 | -136 | - | - |
| 2331 | 0.10 | 179 | 508.99 | 22 | 54.60 | 23 | - | - |
| 2332 | 94.83 | 179 | $(6.88)10^{-3}$ | 24 | 0.62 | -157 | - | - |
| 2333 | 2.72 | -1 | 0.16 | 22 | - | - | - | - |
| 3311 | - | - | $(6.48)10^{-3}$ | 44 | 0.05 | 46 | - | - |
| 3312 | $(1.18)10^{-3}$ | -159 | 0.61 | -159 | $(4.58)10^{4}$ | -157 | - | - |
| 3313 | 0.10 | -3 | $(1.23)10^{4}$ | 22 | 2.24 | -156 | - | - |
| 3322 | 0.11 | -2 | - | - | 0.05 | -134 | - | - |
| 3323 | $(2.30)10^{3}$ | 179 | $(8.60)10^{-3}$ | 45 | 0.02 | 45 | - | - |
| 3333 | 0.11 | 178 | $(6.51)10^{-3}$ | -136 | - | - | - | - |

Table 6: The modulus (in the units of $\text{TeV}^2$) and the argument (in degrees) of $P_a^{ij}(\Lambda)$ in Warsaw-up basis for meson systems at scale $\Lambda = 5\,\text{TeV}$ is shown.

| $[\mathcal{C}^{(8)}_{qd}]_{ijkl}$**(Warsaw-down)** | | | | | | | | |
|---|---|---|---|---|---|---|---|---|
| $ijkl$ | $\lvert P^{sb}_a\rvert$ | $\arg(P^{sb}_a)$ | $\lvert P^{db}_a\rvert$ | $\arg(P^{db}_a)$ | $\lvert P^{sd}_a\rvert$ | $\arg(P^{sd}_a)$ | $\lvert P^{cu}_a\rvert$ | $\arg(P^{cu}_a)$ |
| 1111 | - | - | - | - | $(1.53)10^{-3}$ | 45 | - | - |
| 1112 | - | - | 0.01 | -159 | $(1.15)10^{3}$ | -153 | - | - |
| 1113 | - | - | 282.50 | 22 | 0.07 | -156 | - | - |
| 1122 | - | - | - | - | $(1.53)10^{-3}$ | -135 | - | - |
| 1123 | 0.06 | 179 | - | - | - | - | - | - |
| 1211 | - | - | - | - | 83.93 | -79 | - | - |
| 1212 | - | - | 0.06 | -2 | $(1.87)10^{8}$ | 0 | - | - |
| 1213 | - | - | $(1.28)10^{3}$ | 179 | $(9.18)10^{3}$ | 1 | - | - |
| 1221 | - | - | - | - | 0.16 | 46 | - | - |
| 1222 | - | - | - | - | 83.95 | 101 | $(1.00)10^{-3}$ | 180 |
| 1223 | $(7.43)10^{-3}$ | -24 | $(1.46)10^{-3}$ | -158 | 0.01 | 24 | $(2.36)10^{-3}$ | 179 |
| 1231 | - | - | 0.03 | -135 | - | - | - | - |
| 1232 | 11.56 | 22 | - | - | 98.61 | -158 | - | - |
| 1233 | - | - | - | - | $(7.38)10^{-3}$ | -157 | $(1.87)10^{-3}$ | -107 |
| 1311 | - | - | 0.91 | 21 | 0.36 | -156 | - | - |
| 1312 | - | - | 79.78 | 179 | $(3.18)10^{5}$ | 1 | - | - |
| 1313 | - | - | $(1.63)10^{6}$ | 0 | 15.60 | 2 | - | - |
| 1321 | - | - | - | - | 3.67 | -135 | - | - |
| 1322 | - | - | 0.02 | 22 | 0.36 | 24 | - | - |
| 1323 | 0.65 | 157 | 1.85 | 23 | - | - | - | - |
| 1331 | - | - | 0.78 | 44 | - | - | - | - |
| 1332 | 0.14 | -159 | - | - | 0.17 | -157 | - | - |
| 1333 | - | - | 0.88 | -159 | - | - | - | - |
| 2211 | - | - | - | - | $(3.42)10^{-3}$ | -135 | - | - |
| 2212 | - | - | - | - | $(2.81)10^{3}$ | 24 | - | - |
| 2213 | - | - | 0.44 | 22 | 0.15 | 23 | - | - |
| 2222 | $(2.63)10^{-3}$ | -2 | - | - | $(3.42)10^{-3}$ | 45 | - | - |
| 2223 | 52.80 | 179 | - | - | $(1.58)10^{-3}$ | -136 | - | - |
| 2233 | $(2.53)10^{-3}$ | 178 | - | - | - | - | - | - |
| 2311 | $(4.30)10^{-3}$ | 179 | - | - | 0.08 | 44 | - | - |
| 2312 | - | - | $(1.17)10^{-3}$ | -158 | 24.16 | 24 | - | - |
| 2313 | 0.08 | 158 | 22.13 | 23 | $(1.18)10^{-3}$ | 25 | - | - |
| 2321 | 0.04 | 22 | - | - | $(6.98)10^{4}$ | -158 | - | - |
| 2322 | 3.24 | 179 | - | - | 0.08 | -136 | - | - |
| 2323 | $(6.67)10^{4}$ | -0 | - | - | 0.04 | 44 | - | - |
| 2331 | $(1.00)10^{-3}$ | -2 | 3.56 | -159 | 3.42 | -157 | - | - |
| 2332 | 0.66 | -2 | - | - | - | - | - | - |
| 2333 | 3.22 | -1 | - | - | - | - | - | - |
| 3312 | - | - | 0.03 | 21 | 566.14 | -157 | - | - |
| 3313 | - | - | 512.09 | -158 | 0.03 | -156 | - | - |
| 3322 | $(4.71)10^{-3}$ | 178 | - | - | - | - | - | - |
| 3323 | 95.63 | -1 | - | - | - | - | - | - |
| 3333 | $(4.64)10^{-3}$ | -2 | - | - | - | - | - | - |

Table 7: The modulus (in the units of $\text{TeV}^2$) and the argument (in degrees) of $P^{ij}_a(\Lambda)$ in Warsaw-down basis for meson systems at scale $\Lambda = 5\,\text{TeV}$ is shown.

| $[\mathcal{C}_{qd}^{(8)}]_{ijkl}$ **(Warsaw-up)** | | | | | | | | |
|---|---|---|---|---|---|---|---|---|
| $ijkl$ | $\lvert P_a^{sb}\rvert$ | $\arg(P_a^{sb})$ | $\lvert P_a^{db}\rvert$ | $\arg(P_a^{db})$ | $\lvert P_a^{sd}\rvert$ | $\arg(P_a^{sd})$ | $\lvert P_a^{cu}\rvert$ | $\arg(P_a^{cu})$ |
| 1111 | - | - | $(3.01)10^{-3}$ | -51 | 37.42 | -151 | - | - |
| 1112 | - | - | 0.28 | 106 | $(4.10)10^{7}$ | 0 | - | - |
| 1113 | - | - | $(5.64)10^{3}$ | -73 | $(2.00)10^{3}$ | 1 | - | - |
| 1122 | $(2.60)10^{-3}$ | 106 | - | - | 37.42 | 29 | - | - |
| 1123 | 53.14 | -73 | $(6.62)10^{-3}$ | -40 | 21.56 | -158 | - | - |
| 1133 | $(2.59)10^{-3}$ | -74 | $(2.91)10^{-3}$ | 129 | $(1.61)10^{-3}$ | -157 | - | - |
| 1211 | - | - | 0.04 | 23 | 74.07 | -93 | - | - |
| 1212 | - | - | 3.22 | 179 | $(1.78)10^{8}$ | 0 | - | - |
| 1213 | $(2.14)10^{-3}$ | -87 | $(6.57)10^{4}$ | 0 | $(8.71)10^{3}$ | 1 | - | - |
| 1221 | - | - | 0.06 | -74 | $(9.43)10^{6}$ | 180 | - | - |
| 1222 | 0.04 | 161 | - | - | 74.07 | 87 | $(1.11)10^{-3}$ | 180 |
| 1223 | 619.77 | 0 | 0.07 | 20 | 4.97 | 22 | $(2.50)10^{-3}$ | 180 |
| 1231 | $(2.28)10^{-3}$ | -70 | $(1.29)10^{3}$ | 107 | 461.75 | -179 | - | - |
| 1232 | 230.74 | -73 | $(1.75)10^{-3}$ | -92 | 93.53 | -158 | - | - |
| 1233 | 0.04 | -19 | 0.03 | -157 | $(6.64)10^{-3}$ | -157 | $(2.08)10^{-3}$ | -107 |
| 1311 | - | - | 0.88 | 21 | 8.10 | 22 | - | - |
| 1312 | - | - | 77.68 | 179 | $(7.26)10^{6}$ | -179 | - | - |
| 1313 | 0.02 | 152 | $(1.58)10^{6}$ | 0 | 355.20 | -178 | - | - |
| 1321 | $(7.85)10^{-3}$ | 22 | $(2.46)10^{-3}$ | 128 | $(3.66)10^{5}$ | 22 | - | - |
| 1322 | 0.73 | 179 | 0.02 | 22 | 8.14 | -158 | - | - |
| 1323 | $(1.49)10^{4}$ | 0 | 1.80 | 23 | 0.19 | -136 | - | - |
| 1331 | $(3.16)10^{-3}$ | 106 | 50.36 | -51 | 17.92 | 23 | - | - |
| 1332 | 9.40 | 106 | $(3.58)10^{-3}$ | 128 | 3.78 | 23 | - | - |
| 1333 | 0.73 | -1 | 0.86 | -159 | - | - | - | - |
| 2211 | - | - | $(8.09)10^{-3}$ | -158 | 56.08 | 19 | - | - |
| 2212 | $(1.45)10^{-3}$ | 21 | 0.74 | -1 | $(4.09)10^{7}$ | 180 | - | - |
| 2213 | 0.13 | 1 | $(1.51)10^{4}$ | 180 | $(2.00)10^{3}$ | -179 | - | - |
| 2222 | 0.13 | 179 | - | - | 56.08 | -161 | - | - |
| 2223 | $(2.69)10^{3}$ | 0 | 0.02 | -165 | 21.52 | 22 | - | - |
| 2233 | 0.13 | -1 | $(7.80)10^{-3}$ | 22 | $(1.61)10^{-3}$ | 23 | - | - |
| 2311 | $(4.19)10^{-3}$ | 179 | 0.20 | -158 | 3.58 | -146 | - | - |
| 2312 | - | - | 17.87 | -1 | $(1.67)10^{6}$ | 1 | - | - |
| 2313 | 0.18 | 170 | $(3.65)10^{5}$ | 180 | 81.70 | 2 | - | - |
| 2321 | 0.03 | 22 | 0.03 | -159 | $(1.59)10^{6}$ | 22 | - | - |
| 2322 | 3.15 | 179 | $(4.88)10^{-3}$ | -158 | 3.59 | 34 | - | - |
| 2323 | $(6.49)10^{4}$ | 0 | 0.41 | -157 | 0.84 | -136 | - | - |
| 2331 | 0.16 | 179 | 587.36 | 22 | 77.82 | 23 | - | - |
| 2332 | 109.64 | 179 | 0.01 | 23 | 0.88 | -157 | - | - |
| 2333 | 3.13 | -1 | 0.18 | 22 | - | - | - | - |
| 3311 | - | - | $(7.66)10^{-3}$ | 44 | 0.07 | 46 | - | - |
| 3312 | $(1.36)10^{-3}$ | -159 | 0.70 | -159 | $(6.52)10^{4}$ | -157 | - | - |
| 3313 | 0.15 | -3 | $(1.42)10^{4}$ | 22 | 3.19 | -156 | - | - |
| 3322 | 0.13 | -2 | - | - | 0.07 | -134 | - | - |
| 3323 | $(2.66)10^{3}$ | 179 | $(7.79)10^{-3}$ | 45 | 0.03 | 45 | - | - |
| 3333 | 0.13 | 178 | $(7.33)10^{-3}$ | -136 | - | - | - | - |

Table 8: The modulus (in the units of $\text{TeV}^2$) and the argument (in degrees) of $P_a^{ij}(\Lambda)$ in Warsaw-up basis for meson systems at scale $\Lambda = 5\,\text{TeV}$ is shown.

| $[\mathcal{C}_{qu}^{(1)}]_{ijkl}$**(Warsaw-down)** | | | | | | | | |
|---|---|---|---|---|---|---|---|---|
| $ijkl$ | $\lvert P_a^{sb}\rvert$ | $\arg(P_a^{sb})$ | $\lvert P_a^{db}\rvert$ | $\arg(P_a^{db})$ | $\lvert P_a^{sd}\rvert$ | $\arg(P_a^{sd})$ | $\lvert P_a^{cu}\rvert$ | $\arg(P_a^{cu})$ |
| 1111 | - | - | - | - | - | - | 0.10 | 0 |
| 1112 | - | - | - | - | - | - | $(1.37)10^{7}$ | -180 |
| 1113 | - | - | - | - | - | - | 0.04 | -1 |
| 1122 | - | - | - | - | - | - | 0.10 | -180 |
| 1133 | - | - | $(1.50)10^{-3}$ | 44 | - | - | - | - |
| 1211 | - | - | - | - | - | - | 1.76 | -0 |
| 1212 | - | - | - | - | - | - | $(5.98)10^{7}$ | -0 |
| 1213 | - | - | - | - | $(5.99)10^{-3}$ | 1 | 0.15 | 179 |
| 1221 | - | - | - | - | - | - | $(3.17)10^{6}$ | -180 |
| 1222 | - | - | - | - | 0.06 | -0 | 1.76 | 180 |
| 1223 | - | - | $(1.05)10^{-3}$ | 50 | 0.69 | -179 | - | - |
| 1231 | - | - | - | - | - | - | $(8.22)10^{-3}$ | -2 |
| 1232 | - | - | - | - | 0.66 | -158 | $(1.49)10^{-3}$ | 8 |
| 1233 | - | - | $(6.86)10^{-3}$ | -159 | 5.47 | 23 | - | - |
| 1311 | - | - | $(7.17)10^{-3}$ | 22 | - | - | $(3.75)10^{-3}$ | -2 |
| 1312 | - | - | - | - | - | - | $(2.67)10^{6}$ | -0 |
| 1313 | - | - | 0.04 | 180 | - | - | $(6.89)10^{-3}$ | -180 |
| 1321 | - | - | - | - | - | - | $(5.27)10^{4}$ | -107 |
| 1322 | - | - | $(7.83)10^{-3}$ | 20 | - | - | $(3.87)10^{-3}$ | 178 |
| 1323 | - | - | 4.29 | -0 | $(1.50)10^{-3}$ | -178 | - | - |
| 1331 | - | - | - | - | - | - | 0.78 | -5 |
| 1332 | - | - | $(7.19)10^{-3}$ | -158 | $(1.96)10^{-3}$ | -157 | 0.83 | -0 |
| 1333 | - | - | 32.78 | -158 | 0.01 | 24 | - | - |
| 2211 | - | - | - | - | - | - | 0.10 | 0 |
| 2212 | - | - | - | - | - | - | $(1.37)10^{7}$ | -0 |
| 2213 | - | - | - | - | - | - | 0.05 | 179 |
| 2222 | - | - | - | - | - | - | 0.10 | -180 |
| 2233 | $(1.33)10^{-3}$ | -2 | - | - | - | - | - | - |
| 2311 | $(1.40)10^{-3}$ | 179 | - | - | - | - | - | - |
| 2312 | - | - | - | - | - | - | $(6.15)10^{5}$ | -0 |
| 2313 | - | - | - | - | - | - | $(1.72)10^{-3}$ | -179 |
| 2321 | - | - | - | - | - | - | $(2.28)10^{5}$ | 73 |
| 2322 | $(1.54)10^{-3}$ | 179 | - | - | - | - | - | - |
| 2323 | 0.80 | -180 | - | - | - | - | - | - |
| 2331 | - | - | - | - | - | - | 9.69 | 0 |
| 2332 | $(1.41)10^{-3}$ | -1 | - | - | - | - | 0.04 | -0 |
| 2333 | 6.61 | -1 | - | - | $(3.20)10^{-3}$ | -135 | - | - |
| 3312 | - | - | - | - | - | - | $(1.02)10^{4}$ | 73 |
| 3313 | - | - | - | - | - | - | $(2.60)10^{-3}$ | -145 |
| 3323 | $(2.13)10^{-3}$ | 179 | $(2.49)10^{-3}$ | -158 | - | - | - | - |
| 3333 | 0.02 | -2 | 0.02 | 44 | - | - | - | - |

Table 9: The modulus (in the units of $\mathrm{TeV}^2$) and the argument (in degrees) of $P_a^{ij}(\Lambda)$ in Warsaw-down basis for meson systems at scale $\Lambda = 5\,\mathrm{TeV}$ is shown.

| $[\mathcal{C}_{qu}^{(1)}]_{ijkl}$**(Warsaw-up)** | | | | | | | | |
|---|---|---|---|---|---|---|---|---|
| $ijkl$ | $\lvert P_a^{sb}\rvert$ | $\arg(P_a^{sb})$ | $\lvert P_a^{db}\rvert$ | $\arg(P_a^{db})$ | $\lvert P_a^{sd}\rvert$ | $\arg(P_a^{sd})$ | $\lvert P_a^{cu}\rvert$ | $\arg(P_a^{cu})$ |
| 1112 | - | - | - | - | - | - | 734.83 | -157 |
| 1113 | - | - | - | - | $(1.25)10^{-3}$ | -0 | - | - |
| 1122 | - | - | - | - | 0.01 | -0 | - | - |
| 1123 | - | - | 0.02 | -73 | 0.29 | -169 | - | - |
| 1133 | $(5.36)10^{-3}$ | -74 | 0.12 | 129 | 1.19 | 23 | - | - |
| 1211 | - | - | - | - | - | - | 2.18 | 0 |
| 1212 | - | - | - | - | - | - | $(6.30)10^{7}$ | -0 |
| 1213 | - | - | $(1.52)10^{-3}$ | -180 | $(5.73)10^{-3}$ | 1 | 0.16 | 180 |
| 1221 | - | - | - | - | - | - | $(8.49)10^{-3}$ | -135 |
| 1222 | - | - | - | - | 0.05 | -0 | 2.19 | -180 |
| 1223 | $(7.64)10^{-3}$ | -180 | 0.18 | 0 | 0.63 | 180 | - | - |
| 1232 | $(2.80)10^{-3}$ | 107 | $(3.44)10^{-3}$ | 112 | 0.59 | -157 | - | - |
| 1233 | 0.07 | -19 | 1.37 | -157 | 4.91 | 23 | - | - |
| 1311 | - | - | $(6.99)10^{-3}$ | 22 | - | - | - | - |
| 1312 | - | - | - | - | - | - | $(8.02)10^{4}$ | -0 |
| 1313 | - | - | 0.04 | -180 | - | - | - | - |
| 1321 | - | - | - | - | - | - | 0.08 | -84 |
| 1322 | - | - | $(7.63)10^{-3}$ | 20 | $(2.19)10^{-3}$ | 180 | - | - |
| 1323 | 0.18 | -180 | 4.18 | -0 | 0.03 | 0 | - | - |
| 1332 | - | - | $(6.95)10^{-3}$ | -157 | 0.02 | 23 | 0.84 | -0 |
| 1333 | 1.47 | -1 | 31.93 | -158 | 0.19 | -157 | - | - |
| 2212 | - | - | - | - | - | - | 729.20 | 22 |
| 2213 | - | - | - | - | $(1.24)10^{-3}$ | 180 | - | - |
| 2222 | - | - | - | - | 0.01 | 180 | - | - |
| 2223 | 0.03 | 180 | 0.04 | -180 | 0.29 | 11 | - | - |
| 2233 | 0.27 | -1 | 0.32 | 22 | 1.19 | -157 | - | - |
| 2311 | $(1.37)10^{-3}$ | 179 | $(1.60)10^{-3}$ | -158 | - | - | - | - |
| 2312 | - | - | - | - | - | - | 0.93 | 22 |
| 2313 | - | - | $(8.35)10^{-3}$ | -0 | - | - | - | - |
| 2321 | - | - | - | - | - | - | $(6.85)10^{3}$ | 73 |
| 2322 | $(1.50)10^{-3}$ | 179 | $(1.75)10^{-3}$ | -160 | $(1.01)10^{-3}$ | 11 | - | - |
| 2323 | 0.78 | -180 | 0.96 | 180 | 0.01 | -158 | - | - |
| 2331 | - | - | - | - | - | - | 0.84 | 180 |
| 2332 | $(2.59)10^{-3}$ | -1 | $(3.03)10^{-3}$ | 22 | 0.01 | -157 | - | - |
| 2333 | 6.41 | -1 | 7.51 | 22 | 0.09 | 34 | - | - |
| 3312 | - | - | - | - | - | - | 8.72 | 73 |
| 3323 | 0.03 | -1 | 0.04 | 22 | - | - | - | - |
| 3333 | 0.26 | 178 | 0.29 | -136 | $(1.81)10^{-3}$ | -134 | - | - |

Table 10: The modulus (in the units of $\mathrm{TeV}^2$) and the argument (in degrees) of $P_a^{ij}(\Lambda)$ in Warsaw-up basis for meson systems at scale $\Lambda = 5\,\mathrm{TeV}$ is shown.

| $[\mathcal{C}_{qu}^{(8)}]_{ijkl}$**(Warsaw-down)** | | | | | | | | |
|---|---|---|---|---|---|---|---|---|
| $ijkl$ | $\lvert P_a^{sb}\rvert$ | $\arg(P_a^{sb})$ | $\lvert P_a^{db}\rvert$ | $\arg(P_a^{db})$ | $\lvert P_a^{sd}\rvert$ | $\arg(P_a^{sd})$ | $\lvert P_a^{cu}\rvert$ | $\arg(P_a^{cu})$ |
| 1111 | - | - | - | - | - | - | 0.18 | 0 |
| 1112 | - | - | - | - | - | - | $(1.80)10^{7}$ | -180 |
| 1113 | - | - | - | - | - | - | 0.06 | 2 |
| 1122 | - | - | - | - | - | - | 0.18 | -180 |
| 1133 | - | - | $(5.60)10^{-3}$ | 44 | - | - | - | - |
| 1211 | - | - | - | - | $(2.57)10^{-3}$ | -158 | 3.09 | -0 |
| 1212 | - | - | - | - | - | - | $(7.82)10^{7}$ | -0 |
| 1213 | - | - | - | - | $(2.59)10^{-3}$ | 1 | 0.19 | 179 |
| 1221 | - | - | - | - | - | - | $(4.14)10^{6}$ | -180 |
| 1222 | - | - | - | - | 0.02 | -2 | 3.09 | 180 |
| 1223 | - | - | $(2.13)10^{-3}$ | 30 | 0.30 | -179 | - | - |
| 1231 | - | - | - | - | - | - | 0.01 | -4 |
| 1232 | - | - | - | - | 0.29 | -158 | $(2.65)10^{-3}$ | 3 |
| 1233 | $(1.12)10^{-3}$ | -159 | 0.03 | -159 | 2.29 | 23 | - | - |
| 1311 | - | - | 0.02 | 22 | - | - | $(6.57)10^{-3}$ | -2 |
| 1312 | - | - | - | - | - | - | $(3.49)10^{6}$ | -0 |
| 1313 | - | - | 0.02 | 180 | - | - | $(8.83)10^{-3}$ | -180 |
| 1321 | - | - | - | - | - | - | $(6.89)10^{4}$ | -107 |
| 1322 | - | - | 0.02 | 22 | - | - | $(6.78)10^{-3}$ | 178 |
| 1323 | - | - | 1.86 | -0 | - | - | - | - |
| 1331 | - | - | - | - | - | - | 2.00 | -5 |
| 1332 | - | - | $(2.96)10^{-3}$ | -158 | $(1.44)10^{-3}$ | -157 | 1.49 | -0 |
| 1333 | - | - | 13.09 | -158 | $(9.38)10^{-3}$ | 25 | - | - |
| 2211 | - | - | - | - | - | - | 0.18 | 0 |
| 2212 | - | - | - | - | - | - | $(1.80)10^{7}$ | -0 |
| 2213 | - | - | - | - | - | - | 0.32 | 179 |
| 2222 | - | - | - | - | - | - | 0.18 | -180 |
| 2233 | $(5.01)10^{-3}$ | -2 | - | - | - | - | - | - |
| 2311 | $(4.34)10^{-3}$ | 179 | - | - | - | - | - | - |
| 2312 | - | - | - | - | - | - | $(8.04)10^{5}$ | -0 |
| 2313 | - | - | - | - | - | - | $(2.37)10^{-3}$ | -178 |
| 2321 | - | - | - | - | - | - | $(2.99)10^{5}$ | 73 |
| 2322 | $(4.40)10^{-3}$ | 179 | - | - | - | - | - | - |
| 2323 | 0.35 | -180 | - | - | - | - | - | - |
| 2331 | - | - | - | - | - | - | 13.29 | 3 |
| 2332 | - | - | - | - | - | - | 0.06 | -0 |
| 2333 | 2.66 | -1 | - | - | $(2.14)10^{-3}$ | -136 | - | - |
| 3312 | - | - | - | - | - | - | $(1.33)10^{4}$ | 73 |
| 3313 | - | - | - | - | - | - | $(5.35)10^{-3}$ | -138 |
| 3323 | $(1.65)10^{-3}$ | 179 | $(1.93)10^{-3}$ | -158 | - | - | - | - |
| 3333 | 0.01 | -2 | 0.01 | 44 | - | - | - | - |

Table 11: The modulus (in the units of $\text{TeV}^2$) and the argument (in degrees) of $P_a^{ij}(\Lambda)$ in Warsaw-down basis for meson systems at scale $\Lambda = 5\,\text{TeV}$ is shown.

| $[\mathcal{C}_{qu}^{(8)}]_{ijkl}$ **(Warsaw-up)** | | | | | | | | |
|---|---|---|---|---|---|---|---|---|
| $ijkl$ | $\lvert P_a^{sb}\rvert$ | $\arg(P_a^{sb})$ | $\lvert P_a^{db}\rvert$ | $\arg(P_a^{db})$ | $\lvert P_a^{sd}\rvert$ | $\arg(P_a^{sd})$ | $\lvert P_a^{cu}\rvert$ | $\arg(P_a^{cu})$ |
| 1112 | - | - | - | - | - | - | 960.94 | -157 |
| 1122 | - | - | - | - | $(5.31)10^{-3}$ | -2 | - | - |
| 1123 | - | - | $(6.49)10^{-3}$ | -73 | 0.13 | -169 | - | - |
| 1133 | $(2.21)10^{-3}$ | -76 | 0.05 | 129 | 0.50 | 23 | - | - |
| 1211 | - | - | - | - | $(2.31)10^{-3}$ | -158 | 3.83 | 0 |
| 1212 | - | - | - | - | - | - | $(8.24)10^{7}$ | -0 |
| 1213 | - | - | - | - | $(2.48)10^{-3}$ | 1 | 0.21 | 180 |
| 1221 | - | - | - | - | - | - | 0.01 | -135 |
| 1222 | - | - | - | - | 0.02 | -2 | 3.83 | -180 |
| 1223 | $(3.39)10^{-3}$ | -180 | 0.08 | 1 | 0.27 | 180 | - | - |
| 1232 | $(1.21)10^{-3}$ | 107 | $(1.49)10^{-3}$ | 112 | 0.26 | -157 | - | - |
| 1233 | 0.03 | -19 | 0.58 | -157 | 2.06 | 23 | - | - |
| 1311 | - | - | 0.02 | 22 | - | - | - | - |
| 1312 | - | - | - | - | - | - | $(1.04)10^{5}$ | -0 |
| 1313 | - | - | 0.02 | -180 | - | - | - | - |
| 1321 | - | - | - | - | - | - | 0.10 | -84 |
| 1322 | - | - | 0.02 | 22 | - | - | - | - |
| 1323 | 0.08 | -180 | 1.82 | -0 | 0.01 | 0 | - | - |
| 1332 | - | - | $(2.85)10^{-3}$ | -156 | $(9.34)10^{-3}$ | 23 | 1.50 | -0 |
| 1333 | 0.59 | -1 | 12.75 | -158 | 0.08 | -156 | - | - |
| 2212 | - | - | - | - | - | - | 953.58 | 22 |
| 2222 | - | - | - | - | $(5.30)10^{-3}$ | 178 | - | - |
| 2223 | 0.01 | 180 | 0.02 | -179 | 0.13 | 11 | - | - |
| 2233 | 0.11 | -1 | 0.13 | 22 | 0.50 | -157 | - | - |
| 2311 | $(4.22)10^{-3}$ | 179 | $(4.95)10^{-3}$ | -158 | - | - | - | - |
| 2312 | - | - | - | - | - | - | 1.21 | 22 |
| 2313 | - | - | $(3.63)10^{-3}$ | -0 | - | - | - | - |
| 2321 | - | - | - | - | - | - | $(8.96)10^{3}$ | 73 |
| 2322 | $(4.28)10^{-3}$ | 179 | $(5.01)10^{-3}$ | -159 | - | - | - | - |
| 2323 | 0.34 | -180 | 0.42 | 180 | $(4.72)10^{-3}$ | -158 | - | - |
| 2331 | - | - | - | - | - | - | 1.50 | 180 |
| 2332 | $(1.08)10^{-3}$ | -1 | $(1.25)10^{-3}$ | 23 | $(4.41)10^{-3}$ | -157 | - | - |
| 2333 | 2.58 | -1 | 3.03 | 22 | 0.04 | 34 | - | - |
| 3312 | - | - | - | - | - | - | 11.41 | 73 |
| 3323 | 0.01 | -1 | 0.01 | 22 | - | - | - | - |
| 3333 | 0.10 | 178 | 0.11 | -136 | - | - | - | - |

Table 12: The modulus (in the units of $\text{TeV}^2$) and the argument (in degrees) of $P_a^{ij}(\Lambda)$ in Warsaw-up basis for meson systems at scale $\Lambda = 5\,\text{TeV}$ is shown.

| | | | | $[\mathcal{C}_{dd}]_{ijkl}$ | | | | |
|---|---|---|---|---|---|---|---|---|
| $ijkl$ | $\lvert P_a^{sb}\rvert$ | $\arg(P_a^{sb})$ | $\lvert P_a^{db}\rvert$ | $\arg(P_a^{db})$ | $\lvert P_a^{sd}\rvert$ | $\arg(P_a^{sd})$ | $\lvert P_a^{cu}\rvert$ | $\arg(P_a^{cu})$ |
| 1112 | - | - | - | - | 0.06 | 176 | - | - |
| 1113 | - | - | 0.11 | 21 | - | - | - | - |
| 1123 | $(5.60)10^{-3}$ | -1 | - | - | - | - | - | - |
| 1212 | - | - | - | - | $(9.18)10^{5}$ | -180 | - | - |
| 1213 | - | - | 11.78 | -1 | 44.93 | -179 | - | - |
| 1222 | - | - | - | - | 2.04 | -157 | - | - |
| 1223 | - | - | 0.27 | 22 | - | - | - | - |
| 1231 | 0.05 | 179 | - | - | - | - | - | - |
| 1232 | $(5.45)10^{-3}$ | -158 | - | - | 0.47 | 22 | - | - |
| 1233 | - | - | - | - | 0.14 | 22 | - | - |
| 1313 | - | - | $(2.40)10^{5}$ | -180 | $(2.19)10^{-3}$ | -178 | - | - |
| 1322 | - | - | 0.03 | -158 | - | - | - | - |
| 1323 | 0.01 | -23 | 0.27 | -157 | - | - | - | - |
| 1332 | - | - | - | - | 1.19 | -158 | - | - |
| 1333 | - | - | 0.36 | 22 | - | - | - | - |
| 2223 | 0.46 | -1 | - | - | - | - | - | - |
| 2323 | $(1.03)10^{4}$ | 180 | - | - | - | - | - | - |
| 2333 | 0.55 | 179 | - | - | - | - | - | - |

Table 13: The modulus (in the units of $\text{TeV}^2$) and the argument (in degrees) of $P_a^{ij}(\Lambda)$ in Warsaw-down basis for meson systems at scale $\Lambda = 5\,\text{TeV}$ is shown.

| | | | | $[\mathcal{C}_{uu}]_{ijkl}$ | | | | |
|---|---|---|---|---|---|---|---|---|
| $ijkl$ | $\lvert P_a^{sb}\rvert$ | $\arg(P_a^{sb})$ | $\lvert P_a^{db}\rvert$ | $\arg(P_a^{db})$ | $\lvert P_a^{sd}\rvert$ | $\arg(P_a^{sd})$ | $\lvert P_a^{cu}\rvert$ | $\arg(P_a^{cu})$ |
| 1112 | - | - | - | - | - | - | 0.53 | 180 |
| 1212 | - | - | - | - | - | - | $(5.03)10^{6}$ | 180 |
| 1213 | - | - | - | - | - | - | 0.01 | -0 |
| 1222 | - | - | - | - | - | - | 0.53 | 0 |
| 1233 | - | - | - | - | - | - | $(2.74)10^{-3}$ | 49 |
| 2333 | - | - | $(1.15)10^{-3}$ | 22 | - | - | - | - |
| 3333 | $(7.86)10^{-3}$ | 178 | $(8.77)10^{-3}$ | -136 | - | - | - | - |

Table 14: The modulus (in the units of $\text{TeV}^2$) and the argument (in degrees) of $P_a^{ij}(\Lambda)$ in Warsaw-down basis for meson systems at scale $\Lambda = 5\,\text{TeV}$ is shown.

| $[\mathcal{C}^{(1)}_{ud}]_{ijkl}$ | | | | | | | | |
|---|---|---|---|---|---|---|---|---|
| $ijkl$ | $\lvert P_a^{sb}\rvert$ | $\arg(P_a^{sb})$ | $\lvert P_a^{db}\rvert$ | $\arg(P_a^{db})$ | $\lvert P_a^{sd}\rvert$ | $\arg(P_a^{sd})$ | $\lvert P_a^{cu}\rvert$ | $\arg(P_a^{cu})$ |
| 1112 | - | - | - | - | 0.20 | -157 | - | - |
| 1113 | - | - | 0.04 | 22 | - | - | - | - |
| 1123 | $(7.68)10^{-3}$ | 179 | - | - | - | - | - | - |
| 1212 | - | - | - | - | 0.04 | 0 | $(3.73)10^{-3}$ | -0 |
| 1213 | - | - | - | - | - | - | $(8.37)10^{-3}$ | -0 |
| 1221 | - | - | - | - | $(2.10)10^{-3}$ | 180 | $(1.97)10^{-4}$ | -180 |
| 1222 | - | - | - | - | - | - | 0.02 | -0 |
| 1223 | - | - | - | - | - | - | 0.04 | -0 |
| 1231 | - | - | - | - | - | - | $(1.65)10^{-4}$ | -107 |
| 1232 | - | - | - | - | - | - | 0.01 | 73 |
| 1233 | - | - | - | - | - | - | 0.03 | 73 |
| 1312 | - | - | - | - | 0.45 | -179 | - | - |
| 1313 | - | - | 0.13 | 0 | - | - | - | - |
| 1321 | - | - | - | - | 0.02 | 22 | - | - |
| 1323 | $(1.26)10^{-3}$ | 0 | - | - | - | - | - | - |
| 2212 | - | - | - | - | 4.76 | -179 | - | - |
| 2213 | - | - | 0.04 | 23 | $(2.33)10^{-4}$ | -178 | - | - |
| 2223 | $(7.23)10^{-3}$ | 179 | - | - | - | - | - | - |
| 2311 | - | - | - | - | $(1.13)10^{-4}$ | -146 | - | - |
| 2312 | - | - | $(7.58)10^{-4}$ | -1 | 51.92 | 1 | - | - |
| 2313 | - | - | 15.51 | 180 | $(2.54)10^{-3}$ | 2 | - | - |
| 2321 | - | - | - | - | 49.44 | 22 | - | - |
| 2322 | $(1.34)10^{-4}$ | 179 | - | - | $(1.13)10^{-4}$ | 34 | - | - |
| 2323 | 2.75 | 0 | - | - | - | - | - | - |
| 2331 | - | - | 0.03 | 22 | $(2.41)10^{-3}$ | 23 | - | - |
| 2332 | $(4.93)10^{-3}$ | 179 | - | - | - | - | - | - |
| 2333 | $(1.33)10^{-4}$ | -1 | - | - | - | - | - | - |
| 3311 | - | - | - | - | $(5.55)10^{-4}$ | 46 | - | - |
| 3312 | - | - | $(6.87)10^{-3}$ | -159 | 488.57 | -157 | - | - |
| 3313 | $(1.07)10^{-4}$ | -8 | 140.45 | 22 | 0.02 | -156 | - | - |
| 3322 | $(1.28)10^{-3}$ | -2 | - | - | $(5.55)10^{-4}$ | -134 | - | - |
| 3323 | 26.15 | 179 | $(1.55)10^{-4}$ | 44 | $(2.56)10^{-4}$ | 45 | - | - |
| 3333 | $(1.27)10^{-3}$ | 178 | - | - | - | - | - | - |

Table 15: The modulus (in the units of $\mathrm{TeV}^2$) and the argument (in degrees) of $P_a^{ij}(\Lambda)$ in Warsaw-down basis for meson systems at scale $\Lambda = 5\,\mathrm{TeV}$ is shown.

| $[\mathcal{C}_{ud}^{(8)}]_{ijkl}$ | | | | | | | | |
|---|---|---|---|---|---|---|---|---|
| $ijkl$ | $\|P_a^{sb}\|$ | $\arg(P_a^{sb})$ | $\|P_a^{db}\|$ | $\arg(P_a^{db})$ | $\|P_a^{sd}\|$ | $\arg(P_a^{sd})$ | $\|P_a^{cu}\|$ | $\arg(P_a^{cu})$ |
| 1112 | - | - | - | - | 0.62 | -158 | - | - |
| 1113 | - | - | 0.14 | 22 | - | - | - | - |
| 1123 | 0.03 | 179 | - | - | - | - | - | - |
| 1212 | - | - | - | - | 0.08 | 0 | $(6.44)10^{-3}$ | -0 |
| 1213 | - | - | - | - | - | - | 0.01 | -0 |
| 1221 | - | - | - | - | $(4.23)10^{-3}$ | 180 | $(3.41)10^{-4}$ | -180 |
| 1222 | - | - | - | - | - | - | 0.03 | 0 |
| 1223 | - | - | - | - | - | - | 0.07 | -0 |
| 1231 | - | - | - | - | - | - | $(2.85)10^{-4}$ | -107 |
| 1232 | - | - | - | - | - | - | 0.03 | 73 |
| 1233 | - | - | - | - | - | - | 0.06 | 73 |
| 1312 | - | - | - | - | 0.90 | -179 | - | - |
| 1313 | - | - | 0.19 | 0 | - | - | - | - |
| 1321 | - | - | - | - | 0.05 | 22 | - | - |
| 1323 | $(1.77)10^{-3}$ | 0 | - | - | - | - | - | - |
| 2212 | - | - | - | - | 9.77 | -179 | - | - |
| 2213 | - | - | 0.13 | 22 | $(4.78)10^{-4}$ | -178 | - | - |
| 2223 | 0.03 | 179 | - | - | - | - | - | - |
| 2311 | - | - | - | - | $(2.27)10^{-4}$ | -146 | - | - |
| 2312 | - | - | $(1.06)10^{-3}$ | -1 | 104.07 | 1 | - | - |
| 2313 | - | - | 21.71 | 180 | $(5.09)10^{-3}$ | 2 | - | - |
| 2321 | - | - | - | - | 99.10 | 22 | - | - |
| 2322 | $(1.79)10^{-4}$ | 179 | - | - | $(2.27)10^{-4}$ | 34 | - | - |
| 2323 | 3.86 | 0 | - | - | - | - | - | - |
| 2331 | - | - | 0.04 | 22 | $(4.84)10^{-3}$ | 23 | - | - |
| 2332 | $(6.93)10^{-3}$ | 179 | - | - | - | - | - | - |
| 2333 | $(1.97)10^{-4}$ | -1 | - | - | - | - | - | - |
| 3311 | - | - | - | - | $(1.07)10^{-3}$ | 46 | - | - |
| 3312 | - | - | $(9.66)10^{-3}$ | -159 | 941.57 | -157 | - | - |
| 3313 | $(3.05)10^{-4}$ | -5 | 197.44 | 22 | 0.05 | -156 | - | - |
| 3322 | $(1.75)10^{-3}$ | -2 | - | - | $(1.07)10^{-3}$ | -134 | - | - |
| 3323 | 36.87 | 179 | $(2.09)10^{-4}$ | 45 | $(4.94)10^{-4}$ | 45 | - | - |
| 3333 | $(1.85)10^{-3}$ | 178 | $(1.58)10^{-4}$ | -136 | - | - | - | - |

Table 16: The modulus (in the units of $\text{TeV}^2$) and the argument (in degrees) of $P_a^{ij}(\Lambda)$ in Warsaw-down basis for meson systems at scale $\Lambda = 5\,\text{TeV}$ is shown.

| $[\mathcal{C}^{(1)}_{quqd}]_{ijkl}$ **(Warsaw-down)** | | | | | | | | |
|---|---|---|---|---|---|---|---|---|
| $ijkl$ | $\vert P_a^{sb}\vert$ | $\arg(P_a^{sb})$ | $\vert P_a^{db}\vert$ | $\arg(P_a^{db})$ | $\vert P_a^{sd}\vert$ | $\arg(P_a^{sd})$ | $\vert P_a^{cu}\vert$ | $\arg(P_a^{cu})$ |
| 1111 | - | - | - | - | - | - | 0.01 | -180 |
| 1112 | - | - | - | - | - | - | 0.06 | -180 |
| 1113 | - | - | - | - | - | - | 0.05 | -107 |
| 1121 | - | - | - | - | - | - | 0.06 | 0 |
| 1122 | - | - | - | - | - | - | 0.27 | 0 |
| 1123 | - | - | - | - | - | - | 0.22 | 73 |
| 1131 | - | - | - | - | - | - | $(2.55)10^{-3}$ | 0 |
| 1132 | - | - | - | - | - | - | 0.01 | -0 |
| 1133 | - | - | - | - | - | - | 0.01 | 73 |
| 1212 | - | - | - | - | 0.59 | -180 | 0.01 | 180 |
| 1213 | - | - | - | - | - | - | 0.02 | 180 |
| 1222 | - | - | - | - | - | - | $(2.33)10^{-3}$ | 180 |
| 1223 | - | - | - | - | - | - | $(5.24)10^{-3}$ | 180 |
| 1312 | - | - | - | - | 6.62 | 1 | - | - |
| 1313 | - | - | 1.48 | -180 | - | - | - | - |
| 1321 | - | - | - | - | $(1.39)10^{-3}$ | 44 | - | - |
| 1322 | - | - | - | - | 0.01 | -178 | - | - |
| 1331 | - | - | $(1.88)10^{-3}$ | -136 | - | - | - | - |
| 1332 | - | - | - | - | 1.03 | -180 | - | - |
| 1333 | - | - | 0.02 | -169 | - | - | - | - |
| 2111 | - | - | - | - | - | - | 0.06 | 0 |
| 2112 | - | - | - | - | - | - | 0.27 | 0 |
| 2113 | - | - | - | - | - | - | 0.22 | 73 |
| 2121 | - | - | - | - | 0.02 | -180 | 0.25 | 180 |
| 2122 | - | - | - | - | - | - | 1.17 | 180 |
| 2123 | - | - | - | - | - | - | 0.98 | -107 |
| 2131 | - | - | - | - | - | - | 0.01 | -180 |
| 2132 | - | - | - | - | - | - | 0.05 | 180 |
| 2133 | - | - | - | - | - | - | 0.04 | -107 |
| 2212 | - | - | - | - | - | - | $(2.33)10^{-3}$ | 180 |
| 2213 | - | - | - | - | - | - | $(5.24)10^{-3}$ | 180 |
| 2221 | - | - | - | - | 2.75 | -0 | - | - |
| 2223 | - | - | - | - | - | - | $(1.20)10^{-3}$ | 180 |
| 2231 | - | - | - | - | $(4.05)10^{-3}$ | 1 | - | - |
| 2312 | - | - | - | - | 0.02 | -178 | - | - |
| 2321 | - | - | - | - | 29.57 | -158 | - | - |
| 2323 | 1.24 | 180 | - | - | - | - | - | - |
| 2331 | - | - | $(8.46)10^{-3}$ | -159 | 1.07 | -179 | - | - |
| 2332 | $(1.60)10^{-3}$ | -2 | - | - | - | - | - | - |
| 2333 | $(3.97)10^{-3}$ | -180 | - | - | - | - | - | - |
| 3111 | - | - | - | - | - | - | $(2.85)10^{-3}$ | -3 |
| 3112 | - | - | - | - | - | - | 0.01 | -1 |
| 3113 | - | - | - | - | - | - | $(9.99)10^{-3}$ | 71 |
| 3121 | - | - | - | - | - | - | 0.01 | 179 |
| 3122 | - | - | - | - | - | - | 0.05 | 180 |
| 3123 | - | - | - | - | - | - | 0.04 | -108 |
| 3131 | - | - | 0.01 | -180 | - | - | - | - |
| 3132 | - | - | - | - | - | - | $(2.33)10^{-3}$ | -180 |
| 3133 | - | - | - | - | - | - | $(1.94)10^{-3}$ | -107 |
| 3221 | - | - | $(1.07)10^{-3}$ | 174 | $(5.60)10^{-3}$ | 1 | - | - |
| 3231 | - | - | 1.29 | -0 | - | - | - | - |
| 3232 | 0.23 | -180 | - | - | - | - | - | - |
| 3312 | - | - | - | - | 69.59 | 180 | - | - |
| 3313 | - | - | 0.01 | -180 | - | - | - | - |
| 3321 | - | - | $(3.34)10^{-3}$ | 24 | 69.74 | -180 | - | - |
| 3323 | 0.01 | 180 | - | - | - | - | - | - |
| 3331 | $(7.47)10^{-3}$ | 178 | 13.54 | -158 | $(1.36)10^{-3}$ | 24 | - | - |
| 3332 | 2.52 | -1 | - | - | - | - | - | - |

Table 17: The modulus (in the units of $\mathrm{TeV}^2$) and the argument (in degrees) of $P_a^{ij}(\Lambda)$ in Warsaw-down basis for meson systems at scale $\Lambda = 5\,\mathrm{TeV}$ is shown.

| $[\mathcal{C}^{(1)}_{quqd}]_{ijkl}$**(Warsaw-up)** | | | | | | | | |
|---|---|---|---|---|---|---|---|---|
| $ijkl$ | $\lvert P_a^{sb}\rvert$ | $\arg(P_a^{sb})$ | $\lvert P_a^{db}\rvert$ | $\arg(P_a^{db})$ | $\lvert P_a^{sd}\rvert$ | $\arg(P_a^{sd})$ | $\lvert P_a^{cu}\rvert$ | $\arg(P_a^{cu})$ |
| 1111 | - | - | - | - | $(1.20)10^{-3}$ | 180 | - | - |
| 1121 | - | - | - | - | $(5.22)10^{-3}$ | 180 | - | - |
| 1211 | - | - | - | - | 0.14 | 0 | - | - |
| 1212 | - | - | - | - | 0.56 | 180 | 0.01 | -180 |
| 1213 | - | - | - | - | - | - | 0.02 | 180 |
| 1221 | - | - | - | - | 0.60 | -0 | - | - |
| 1222 | - | - | - | - | 0.13 | -0 | - | - |
| 1231 | - | - | $(4.61)10^{-3}$ | -73 | 0.02 | -179 | - | - |
| 1232 | - | - | - | - | $(5.08)10^{-3}$ | -159 | - | - |
| 1311 | - | - | - | - | 1.49 | -160 | - | - |
| 1312 | - | - | - | - | 6.29 | 2 | - | - |
| 1313 | 0.06 | -180 | 1.41 | -180 | - | - | - | - |
| 1321 | - | - | $(2.04)10^{-3}$ | 129 | 6.46 | -158 | - | - |
| 1322 | - | - | - | - | 1.42 | -179 | - | - |
| 1323 | 0.27 | -180 | 0.32 | -0 | - | - | - | - |
| 1331 | - | - | 0.05 | -51 | 6.82 | -1 | - | - |
| 1332 | $(9.40)10^{-3}$ | -74 | - | - | 0.49 | 3 | - | - |
| 1333 | 0.01 | -1 | 0.03 | -164 | - | - | - | - |
| 2111 | - | - | - | - | $(5.22)10^{-3}$ | 180 | - | - |
| 2121 | - | - | - | - | 0.02 | -180 | 0.26 | 180 |
| 2122 | - | - | - | - | - | - | 1.23 | -180 |
| 2123 | - | - | - | - | - | - | 1.03 | -107 |
| 2132 | - | - | - | - | - | - | $(1.44)10^{-3}$ | -180 |
| 2133 | - | - | - | - | - | - | $(1.25)10^{-3}$ | -97 |
| 2211 | - | - | - | - | 0.60 | -0 | - | - |
| 2212 | - | - | - | - | 0.13 | -0 | - | - |
| 2221 | - | - | $(2.23)10^{-3}$ | 0 | 2.61 | -0 | - | - |
| 2222 | - | - | - | - | 0.03 | 180 | - | - |
| 2231 | - | - | 0.05 | 0 | 0.11 | -179 | - | - |
| 2232 | $(9.78)10^{-3}$ | 180 | - | - | $(1.13)10^{-3}$ | 22 | - | - |
| 2311 | - | - | $(2.04)10^{-3}$ | 129 | 6.45 | -158 | - | - |
| 2312 | - | - | - | - | 1.37 | -179 | - | - |
| 2313 | 0.27 | -180 | 0.32 | -0 | - | - | - | - |
| 2321 | - | - | 0.02 | -158 | 27.89 | -158 | - | - |
| 2322 | $(4.59)10^{-3}$ | -1 | - | - | 0.35 | 1 | - | - |
| 2323 | 1.17 | -180 | 0.07 | 180 | - | - | - | - |
| 2331 | 0.02 | 179 | 0.55 | -157 | 28.76 | 1 | - | - |
| 2332 | 0.11 | -1 | $(1.51)10^{-3}$ | 19 | 0.51 | -1 | - | - |
| 2333 | 0.05 | -1 | $(4.57)10^{-3}$ | 24 | - | - | - | - |
| 3122 | - | - | - | - | - | - | $(1.45)10^{-3}$ | -180 |
| 3123 | - | - | - | - | - | - | $(1.34)10^{-3}$ | -108 |
| 3131 | - | - | 0.01 | 180 | - | - | - | - |
| 3211 | - | - | $(4.55)10^{-3}$ | -73 | 0.02 | -179 | - | - |
| 3212 | - | - | - | - | $(5.16)10^{-3}$ | -159 | - | - |
| 3221 | - | - | 0.05 | 0 | 0.11 | -179 | - | - |
| 3222 | $(9.48)10^{-3}$ | 180 | - | - | $(1.08)10^{-3}$ | 22 | - | - |
| 3231 | - | - | 1.29 | 0 | $(4.31)10^{-3}$ | 2 | - | - |
| 3232 | 0.23 | -180 | - | - | - | - | - | - |
| 3311 | - | - | 0.06 | -55 | 364.04 | -0 | - | - |
| 3312 | $(9.11)10^{-3}$ | -71 | - | - | 41.13 | 180 | - | - |
| 3313 | 0.01 | -1 | 0.02 | -169 | - | - | - | - |
| 3321 | 0.04 | 179 | 0.43 | -152 | 844.00 | -0 | - | - |
| 3322 | 0.10 | -2 | $(9.48)10^{-3}$ | 13 | 54.78 | -0 | - | - |
| 3323 | 0.04 | -1 | $(2.47)10^{-3}$ | 27 | - | - | - | - |
| 3331 | 0.05 | -1 | 13.57 | -160 | 0.15 | -159 | - | - |
| 3332 | 2.52 | -1 | $(2.83)10^{-3}$ | -135 | - | - | - | - |
| 3333 | $(2.06)10^{-3}$ | 178 | - | - | - | - | - | - |

Table 18: The modulus (in the units of $\text{TeV}^2$) and the argument (in degrees) of $P_a^{ij}(\Lambda)$ in Warsaw-up basis for meson systems at scale $\Lambda = 5\,\text{TeV}$ is shown.

| $[\mathcal{C}^{(8)}_{quqd}]_{ijkl}$**(Warsaw-down)** | | | | | | | | |
|---|---|---|---|---|---|---|---|---|
| $ijkl$ | $\lvert P_a^{sb}\rvert$ | $\arg(P_a^{sb})$ | $\lvert P_a^{db}\rvert$ | $\arg(P_a^{db})$ | $\lvert P_a^{sd}\rvert$ | $\arg(P_a^{sd})$ | $\lvert P_a^{cu}\rvert$ | $\arg(P_a^{cu})$ |
| 1111 | - | - | - | - | - | - | $(2.20)10^{-3}$ | -180 |
| 1112 | - | - | - | - | - | - | 0.01 | -180 |
| 1113 | - | - | - | - | - | - | $(8.63)10^{-3}$ | -107 |
| 1121 | - | - | - | - | - | - | $(9.56)10^{-3}$ | 0 |
| 1122 | - | - | - | - | - | - | 0.04 | 0 |
| 1123 | - | - | - | - | - | - | 0.04 | 73 |
| 1132 | - | - | - | - | - | - | $(2.00)10^{-3}$ | -0 |
| 1133 | - | - | - | - | - | - | $(1.67)10^{-3}$ | 73 |
| 1212 | - | - | - | - | 0.09 | -180 | $(1.69)10^{-3}$ | 180 |
| 1213 | - | - | - | - | - | - | $(3.80)10^{-3}$ | 180 |
| 1312 | - | - | - | - | 1.06 | 1 | - | - |
| 1313 | - | - | 0.26 | -180 | - | - | - | - |
| 1332 | - | - | - | - | 0.14 | -180 | - | - |
| 1333 | - | - | $(1.15)10^{-3}$ | 24 | - | - | - | - |
| 2111 | - | - | - | - | - | - | $(9.56)10^{-3}$ | 0 |
| 2112 | - | - | - | - | - | - | 0.04 | 0 |
| 2113 | - | - | - | - | - | - | 0.04 | 73 |
| 2121 | - | - | - | - | $(3.82)10^{-3}$ | -180 | 0.04 | 180 |
| 2122 | - | - | - | - | - | - | 0.20 | 180 |
| 2123 | - | - | - | - | - | - | 0.16 | -107 |
| 2131 | - | - | - | - | - | - | $(1.85)10^{-3}$ | 180 |
| 2132 | - | - | - | - | - | - | $(8.71)10^{-3}$ | 180 |
| 2133 | - | - | - | - | - | - | $(7.27)10^{-3}$ | -107 |
| 2221 | - | - | - | - | 0.44 | -0 | - | - |
| 2321 | - | - | - | - | 4.74 | -158 | - | - |
| 2323 | 0.22 | 180 | - | - | - | - | - | - |
| 2331 | - | - | - | - | 0.15 | -178 | - | - |
| 2333 | $(1.04)10^{-3}$ | 179 | - | - | - | - | - | - |
| 3112 | - | - | - | - | - | - | $(2.00)10^{-3}$ | 0 |
| 3113 | - | - | - | - | - | - | $(1.67)10^{-3}$ | 73 |
| 3121 | - | - | - | - | - | - | $(1.85)10^{-3}$ | 180 |
| 3122 | - | - | - | - | - | - | $(8.71)10^{-3}$ | 180 |
| 3123 | - | - | - | - | - | - | $(7.26)10^{-3}$ | -107 |
| 3131 | - | - | $(1.95)10^{-3}$ | -180 | - | - | - | - |
| 3221 | - | - | - | - | $(1.00)10^{-3}$ | 1 | - | - |
| 3231 | - | - | 0.22 | -0 | - | - | - | - |
| 3232 | 0.04 | -180 | - | - | - | - | - | - |
| 3313 | - | - | $(2.79)10^{-3}$ | -158 | - | - | - | - |
| 3321 | - | - | $(1.72)10^{-3}$ | -159 | $(8.61)10^{-3}$ | -157 | - | - |
| 3331 | - | - | 2.38 | -158 | - | - | - | - |
| 3332 | 0.44 | -1 | - | - | - | - | - | - |

Table 19: The modulus (in the units of $\text{TeV}^2$) and the argument (in degrees) of $P_a^{ij}(\Lambda)$ in Warsaw-down basis for meson systems at scale $\Lambda = 5\,\text{TeV}$ is shown.

| $[\mathcal{C}^{(8)}_{quqd}]_{ijkl}$**(Warsaw-up)** | | | | | | | | |
|---|---|---|---|---|---|---|---|---|
| $ijkl$ | $\|P_a^{sb}\|$ | $\arg(P_a^{sb})$ | $\|P_a^{db}\|$ | $\arg(P_a^{db})$ | $\|P_a^{sd}\|$ | $\arg(P_a^{sd})$ | $\|P_a^{cu}\|$ | $\arg(P_a^{cu})$ |
| 1211 | - | - | - | - | 0.02 | -0 | - | - |
| 1212 | - | - | - | - | 0.09 | -180 | $(1.78)10^{-3}$ | 180 |
| 1213 | - | - | - | - | - | - | $(4.00)10^{-3}$ | 180 |
| 1221 | - | - | - | - | 0.10 | -0 | - | - |
| 1222 | - | - | - | - | 0.02 | -0 | - | - |
| 1231 | - | - | - | - | $(3.87)10^{-3}$ | -179 | - | - |
| 1311 | - | - | - | - | 0.24 | -158 | - | - |
| 1312 | - | - | - | - | 1.01 | 1 | - | - |
| 1313 | 0.01 | -180 | 0.25 | -180 | - | - | - | - |
| 1321 | - | - | - | - | 1.03 | -158 | - | - |
| 1322 | - | - | - | - | 0.23 | -179 | - | - |
| 1323 | 0.05 | 180 | 0.06 | -0 | - | - | - | - |
| 1331 | - | - | $(8.65)10^{-3}$ | 129 | 2.03 | 180 | - | - |
| 1332 | $(1.61)10^{-3}$ | -74 | - | - | 0.33 | 1 | - | - |
| 1333 | $(1.85)10^{-3}$ | -1 | $(1.20)10^{-3}$ | -160 | - | - | - | - |
| 2121 | - | - | - | - | $(3.63)10^{-3}$ | -180 | 0.04 | 180 |
| 2122 | - | - | - | - | - | - | 0.21 | 180 |
| 2123 | - | - | - | - | - | - | 0.17 | -107 |
| 2211 | - | - | - | - | 0.10 | -0 | - | - |
| 2212 | - | - | - | - | 0.02 | -0 | - | - |
| 2221 | - | - | - | - | 0.42 | -0 | - | - |
| 2222 | - | - | - | - | $(4.70)10^{-3}$ | 180 | - | - |
| 2231 | - | - | $(9.42)10^{-3}$ | -0 | 0.02 | -179 | - | - |
| 2232 | $(1.67)10^{-3}$ | 180 | - | - | - | - | - | - |
| 2311 | - | - | - | - | 1.04 | -158 | - | - |
| 2312 | - | - | - | - | 0.23 | -179 | - | - |
| 2313 | 0.05 | -180 | 0.06 | -0 | - | - | - | - |
| 2321 | - | - | $(4.24)10^{-3}$ | -158 | 4.49 | -158 | - | - |
| 2322 | - | - | - | - | 0.05 | 1 | - | - |
| 2323 | 0.21 | -180 | 0.01 | 180 | - | - | - | - |
| 2331 | $(1.27)10^{-3}$ | 179 | 0.10 | -158 | 8.95 | 0 | - | - |
| 2332 | 0.02 | -1 | - | - | 0.13 | -0 | - | - |
| 2333 | $(7.85)10^{-3}$ | -1 | - | - | - | - | - | - |
| 3131 | - | - | $(1.95)10^{-3}$ | -180 | - | - | - | - |
| 3211 | - | - | - | - | $(3.86)10^{-3}$ | -179 | - | - |
| 3221 | - | - | $(9.61)10^{-3}$ | 1 | 0.02 | -179 | - | - |
| 3222 | $(1.71)10^{-3}$ | 180 | - | - | - | - | - | - |
| 3231 | - | - | 0.22 | -0 | - | - | - | - |
| 3232 | 0.04 | -180 | - | - | - | - | - | - |
| 3311 | - | - | $(8.75)10^{-3}$ | 129 | 0.04 | 23 | - | - |
| 3312 | $(1.63)10^{-3}$ | -74 | - | - | $(8.89)10^{-3}$ | 23 | - | - |
| 3313 | $(2.07)10^{-3}$ | -1 | $(5.05)10^{-3}$ | -158 | - | - | - | - |
| 3321 | - | - | 0.10 | -158 | 0.18 | 23 | - | - |
| 3322 | 0.02 | -1 | - | - | $(2.07)10^{-3}$ | -157 | - | - |
| 3323 | $(9.01)10^{-3}$ | -1 | $(1.15)10^{-3}$ | 22 | - | - | - | - |
| 3331 | $(1.06)10^{-3}$ | -2 | 2.38 | -158 | $(7.47)10^{-3}$ | -156 | - | - |
| 3332 | 0.44 | -1 | - | - | - | - | - | - |

Table 20: The modulus (in the units of $\text{TeV}^2$) and the argument (in degrees) of $P_a^{ij}(\Lambda)$ in Warsaw-up basis for meson systems at scale $\Lambda = 5\,\text{TeV}$ is shown.

| $[\mathcal{C}^{(1)}_{\phi q}]_{ijkl}$**(Warsaw-down)** | | | | | | | | |
|---|---|---|---|---|---|---|---|---|
| $ijkl$ | $\lvert P_a^{sb}\rvert$ | $\arg(P_a^{sb})$ | $\lvert P_a^{db}\rvert$ | $\arg(P_a^{db})$ | $\lvert P_a^{sd}\rvert$ | $\arg(P_a^{sd})$ | $\lvert P_a^{cu}\rvert$ | $\arg(P_a^{cu})$ |
| 11 | - | - | 0.01 | -136 | - | - | $(1.16)10^{-3}$ | 49 |
| 12 | $(2.07)10^{-3}$ | 21 | 0.05 | 21 | 5.23 | -157 | $(4.80)10^{-3}$ | -131 |
| 13 | - | - | 30.78 | 22 | 0.02 | -156 | - | - |
| 22 | $(9.43)10^{-3}$ | 178 | - | - | - | - | $(1.16)10^{-3}$ | -131 |
| 23 | 6.03 | 179 | - | - | $(4.43)10^{-3}$ | 44 | - | - |
| 33 | 0.01 | 178 | 0.02 | -136 | - | - | - | - |

| $[\mathcal{C}^{(3)}_{\phi q}]_{ijkl}$**(Warsaw-down)** | | | | | | | | |
|---|---|---|---|---|---|---|---|---|
| $ijkl$ | $\lvert P_a^{sb}\rvert$ | $\arg(P_a^{sb})$ | $\lvert P_a^{db}\rvert$ | $\arg(P_a^{db})$ | $\lvert P_a^{sd}\rvert$ | $\arg(P_a^{sd})$ | $\lvert P_a^{cu}\rvert$ | $\arg(P_a^{cu})$ |
| 11 | - | - | 0.14 | 44 | - | - | $(1.20)10^{-3}$ | 49 |
| 12 | 0.03 | -159 | 0.65 | -159 | 13.61 | 23 | $(4.95)10^{-3}$ | -131 |
| 13 | $(1.12)10^{-3}$ | -25 | 68.04 | -158 | 0.13 | 24 | - | - |
| 22 | 0.13 | -2 | - | - | $(1.24)10^{-3}$ | 46 | $(1.20)10^{-3}$ | -131 |
| 23 | 13.40 | -1 | $(7.34)10^{-3}$ | -135 | 0.03 | -135 | - | - |
| 33 | 0.16 | -2 | 0.18 | 44 | - | - | - | - |

| $[\mathcal{C}_{\phi u}]_{ij}$ | | | | | | | | |
|---|---|---|---|---|---|---|---|---|
| $ijkl$ | $\lvert P_a^{sb}\rvert$ | $\arg(P_a^{sb})$ | $\lvert P_a^{db}\rvert$ | $\arg(P_a^{db})$ | $\lvert P_a^{sd}\rvert$ | $\arg(P_a^{sd})$ | $\lvert P_a^{cu}\rvert$ | $\arg(P_a^{cu})$ |
| 12 | - | - | - | - | - | - | 0.05 | 49 |
| 33 | $(3.38)10^{-3}$ | -2 | $(3.77)10^{-3}$ | 44 | - | - | - | - |

| $[\mathcal{C}_{\phi d}]_{ij}$ | | | | | | | | |
|---|---|---|---|---|---|---|---|---|
| $ijkl$ | $\lvert P_a^{sb}\rvert$ | $\arg(P_a^{sb})$ | $\lvert P_a^{db}\rvert$ | $\arg(P_a^{db})$ | $\lvert P_a^{sd}\rvert$ | $\arg(P_a^{sd})$ | $\lvert P_a^{cu}\rvert$ | $\arg(P_a^{cu})$ |
| 12 | - | - | $(8.07)10^{-3}$ | 21 | 611.86 | 23 | - | - |
| 13 | - | - | 165.01 | -158 | 0.03 | 24 | - | - |
| 22 | $(1.51)10^{-3}$ | 178 | - | - | - | - | - | - |
| 23 | 30.74 | -1 | - | - | - | - | - | - |
| 33 | $(1.49)10^{-3}$ | -2 | - | - | - | - | - | - |

Table 21: The modulus (in the units of $\text{TeV}^2$) and the argument (in degrees) of $P_a^{ij}(\Lambda)$ in Warsaw-down basis for meson systems at scale $\Lambda = 5\,\text{TeV}$ is shown.

| $[\mathcal{C}_{\phi q}^{(1)}]_{ijkl}$ **(Warsaw-up)** | | | | | | | | |
|---|---|---|---|---|---|---|---|---|
| $ijkl$ | $\lvert P_a^{sb}\rvert$ | $\arg(P_a^{sb})$ | $\lvert P_a^{db}\rvert$ | $\arg(P_a^{db})$ | $\lvert P_a^{sd}\rvert$ | $\arg(P_a^{sd})$ | $\lvert P_a^{cu}\rvert$ | $\arg(P_a^{cu})$ |
| 11 | $(5.08)10^{-3}$ | 106 | 0.11 | -51 | 1.14 | -157 | - | - |
| 12 | 0.07 | 161 | 1.30 | 23 | 4.70 | -157 | $(5.35)10^{-3}$ | -131 |
| 13 | 1.35 | 179 | 29.97 | 22 | 0.18 | 23 | - | - |
| 22 | 0.26 | 179 | 0.30 | -158 | 1.14 | 23 | - | - |
| 23 | 5.86 | 179 | 6.86 | -158 | 0.08 | -146 | - | - |
| 33 | 0.24 | -2 | 0.26 | 44 | $(1.68)10^{-3}$ | 45 | - | - |

| $[\mathcal{C}_{\phi q}^{(3)}]_{ijkl}$ **(Warsaw-up)** | | | | | | | | |
|---|---|---|---|---|---|---|---|---|
| $ijkl$ | $\lvert P_a^{sb}\rvert$ | $\arg(P_a^{sb})$ | $\lvert P_a^{db}\rvert$ | $\arg(P_a^{db})$ | $\lvert P_a^{sd}\rvert$ | $\arg(P_a^{sd})$ | $\lvert P_a^{cu}\rvert$ | $\arg(P_a^{cu})$ |
| 11 | 0.01 | -74 | 0.30 | 129 | 2.98 | 23 | - | - |
| 12 | 0.18 | -19 | 3.43 | -157 | 12.24 | 23 | $(5.51)10^{-3}$ | -131 |
| 13 | 3.00 | -1 | 66.23 | -158 | 0.40 | -157 | - | - |
| 22 | 0.68 | -1 | 0.79 | 22 | 2.97 | -157 | - | - |
| 23 | 13.01 | -1 | 15.24 | 22 | 0.19 | 34 | - | - |
| 33 | 0.40 | 178 | 0.44 | -136 | $(2.79)10^{-3}$ | -134 | - | - |

Table 22: The modulus (in the units of $\text{TeV}^2$) and the argument (in degrees) of $P_a^{ij}(\Lambda)$ in Warsaw-up basis for meson systems at scale $\Lambda = 5\,\text{TeV}$ is shown.

| $[\mathcal{C}_{lequ}^{(1)}]_{ijkl}$ **(Warsaw-down)** | | | | | | | | |
|---|---|---|---|---|---|---|---|---|
| $ijkl$ | $\lvert P_a^{sb}\rvert$ | $\arg(P_a^{sb})$ | $\lvert P_a^{db}\rvert$ | $\arg(P_a^{db})$ | $\lvert P_a^{sd}\rvert$ | $\arg(P_a^{sd})$ | $\lvert P_a^{cu}\rvert$ | $\arg(P_a^{cu})$ |
| 2213 | - | - | $(2.07)10^{-4}$ | 22 | - | - | - | - |
| 3313 | - | - | $(3.50)10^{-3}$ | 22 | - | - | - | - |
| 3323 | $(6.88)10^{-4}$ | 179 | - | - | - | - | - | - |

Table 23: The modulus (in the units of $\text{TeV}^2$) and the argument (in degrees) of $P_a^{ij}(\Lambda)$ in Warsaw-down basis for meson systems at scale $\Lambda = 5\,\text{TeV}$ is shown.

| $[\mathcal{C}_{lequ}^{(1)}]_{ijkl}$ **(Warsaw-up)** | | | | | | | | |
|---|---|---|---|---|---|---|---|---|
| $ijkl$ | $\lvert P_a^{sb}\rvert$ | $\arg(P_a^{sb})$ | $\lvert P_a^{db}\rvert$ | $\arg(P_a^{db})$ | $\lvert P_a^{sd}\rvert$ | $\arg(P_a^{sd})$ | $\lvert P_a^{cu}\rvert$ | $\arg(P_a^{cu})$ |
| 2213 | - | - | $(2.03)10^{-4}$ | 22 | - | - | - | - |
| 3313 | $(1.54)10^{-4}$ | 179 | $(3.41)10^{-3}$ | 22 | - | - | - | - |
| 3323 | $(6.69)10^{-4}$ | 179 | $(7.83)10^{-4}$ | -158 | - | - | - | - |

Table 24: The modulus (in the units of $\text{TeV}^2$) and the argument (in degrees) of $P_a^{ij}(\Lambda)$ in Warsaw-up basis for meson systems at scale $\Lambda = 5\,\text{TeV}$ is shown.

| $[\mathcal{C}^{(3)}_{lequ}]_{ijkl}$**(Warsaw-down)** | | | | | | | | |
|---|---|---|---|---|---|---|---|---|
| $ijkl$ | $\lvert P_a^{sb}\rvert$ | $\arg(P_a^{sb})$ | $\lvert P_a^{db}\rvert$ | $\arg(P_a^{db})$ | $\lvert P_a^{sd}\rvert$ | $\arg(P_a^{sd})$ | $\lvert P_a^{cu}\rvert$ | $\arg(P_a^{cu})$ |
| 2213 | - | - | $(1.44)10^{-4}$ | 22 | - | - | - | - |
| 3313 | - | - | $(2.43)10^{-3}$ | 22 | - | - | - | - |
| 3323 | $(4.77)10^{-4}$ | 179 | - | - | - | - | - | - |

Table 25: The modulus (in the units of $\text{TeV}^2$) and the argument (in degrees) of $P_a^{ij}(\Lambda)$ in Warsaw-down basis for meson systems at scale $\Lambda = 5\,\text{TeV}$ is shown.

| $[\mathcal{C}^{(3)}_{lequ}]_{ijkl}$**(Warsaw-up)** | | | | | | | | |
|---|---|---|---|---|---|---|---|---|
| $ijkl$ | $\lvert P_a^{sb}\rvert$ | $\arg(P_a^{sb})$ | $\lvert P_a^{db}\rvert$ | $\arg(P_a^{db})$ | $\lvert P_a^{sd}\rvert$ | $\arg(P_a^{sd})$ | $\lvert P_a^{cu}\rvert$ | $\arg(P_a^{cu})$ |
| 2213 | - | - | $(1.40)10^{-4}$ | 22 | - | - | - | - |
| 3313 | $(1.07)10^{-4}$ | 179 | $(2.36)10^{-3}$ | 22 | - | - | - | - |
| 3323 | $(4.64)10^{-4}$ | 179 | $(5.43)10^{-4}$ | -158 | - | - | - | - |

Table 26: The modulus (in the units of $\text{TeV}^2$) and the argument (in degrees) of $P_a^{ij}(\Lambda)$ in Warsaw-up basis for meson systems at scale $\Lambda = 5\,\text{TeV}$ is shown.

| $[\mathcal{C}^{(1)}_{lq}]_{ijkl}$**(Warsaw-down)** | | | | | | | | |
|---|---|---|---|---|---|---|---|---|
| $ijkl$ | $\lvert P_a^{sb}\rvert$ | $\arg(P_a^{sb})$ | $\lvert P_a^{db}\rvert$ | $\arg(P_a^{db})$ | $\lvert P_a^{sd}\rvert$ | $\arg(P_a^{sd})$ | $\lvert P_a^{cu}\rvert$ | $\arg(P_a^{cu})$ |
| 1112 | - | - | $(1.07)10^{-4}$ | 21 | $(7.48)10^{-4}$ | 23 | - | - |
| 1113 | - | - | $(7.08)10^{-3}$ | -158 | - | - | - | - |
| 1123 | $(1.37)10^{-3}$ | -1 | - | - | - | - | - | - |
| 1133 | $(2.52)10^{-4}$ | -2 | $(2.82)10^{-4}$ | 44 | - | - | - | - |
| 2212 | - | - | $(1.07)10^{-4}$ | 21 | $(7.48)10^{-4}$ | 23 | - | - |
| 2213 | - | - | $(7.08)10^{-3}$ | -158 | - | - | - | - |
| 2223 | $(1.37)10^{-3}$ | -1 | - | - | - | - | - | - |
| 2233 | $(2.52)10^{-4}$ | -2 | $(2.82)10^{-4}$ | 44 | - | - | - | - |
| 3312 | - | - | $(1.08)10^{-4}$ | 21 | $(7.35)10^{-4}$ | 23 | - | - |
| 3313 | - | - | $(7.01)10^{-3}$ | -158 | - | - | - | - |
| 3323 | $(1.37)10^{-3}$ | -1 | - | - | - | - | - | - |

Table 27: The modulus (in the units of $\text{TeV}^2$) and the argument (in degrees) of $P_a^{ij}(\Lambda)$ in Warsaw-down basis for meson systems at scale $\Lambda = 5\,\text{TeV}$ is shown.

| $[\mathcal{C}_{lq}^{(1)}]_{ijkl}$**(Warsaw-up)** | | | | | | | | |
|---|---|---|---|---|---|---|---|---|
| $ijkl$ | $\lvert P_a^{sb}\rvert$ | $\arg(P_a^{sb})$ | $\lvert P_a^{db}\rvert$ | $\arg(P_a^{db})$ | $\lvert P_a^{sd}\rvert$ | $\arg(P_a^{sd})$ | $\lvert P_a^{cu}\rvert$ | $\arg(P_a^{cu})$ |
| 1111 | - | - | - | - | $(1.63)10^{-4}$ | 23 | - | - |
| 1112 | - | - | $(1.83)10^{-4}$ | -157 | $(6.72)10^{-4}$ | 23 | - | - |
| 1113 | $(3.12)10^{-4}$ | -1 | $(6.90)10^{-3}$ | -158 | - | - | - | - |
| 1122 | - | - | - | - | $(1.63)10^{-4}$ | -157 | - | - |
| 1123 | $(1.35)10^{-3}$ | -1 | $(1.58)10^{-3}$ | 22 | - | - | - | - |
| 1133 | $(1.95)10^{-4}$ | -2 | $(2.18)10^{-4}$ | 44 | - | - | - | - |
| 2211 | - | - | - | - | $(1.63)10^{-4}$ | 23 | - | - |
| 2212 | - | - | $(1.83)10^{-4}$ | -157 | $(6.71)10^{-4}$ | 23 | - | - |
| 2213 | $(3.12)10^{-4}$ | -1 | $(6.90)10^{-3}$ | -158 | - | - | - | - |
| 2222 | - | - | - | - | $(1.63)10^{-4}$ | -157 | - | - |
| 2223 | $(1.35)10^{-3}$ | -1 | $(1.58)10^{-3}$ | 22 | - | - | - | - |
| 2233 | $(1.95)10^{-4}$ | -2 | $(2.18)10^{-4}$ | 44 | - | - | - | - |
| 3311 | - | - | - | - | $(1.60)10^{-4}$ | 23 | - | - |
| 3312 | - | - | $(1.80)10^{-4}$ | -157 | $(6.60)10^{-4}$ | 23 | - | - |
| 3313 | $(3.09)10^{-4}$ | -1 | $(6.83)10^{-3}$ | -158 | - | - | - | - |
| 3322 | - | - | - | - | $(1.60)10^{-4}$ | -157 | - | - |
| 3323 | $(1.34)10^{-3}$ | -1 | $(1.57)10^{-3}$ | 22 | - | - | - | - |

Table 28: The modulus (in the units of $\text{TeV}^2$) and the argument (in degrees) of $P_a^{ij}(\Lambda)$ in Warsaw-up basis for meson systems at scale $\Lambda = 5\,\text{TeV}$ is shown.

| $[\mathcal{C}_{lq}^{(3)}]_{ijkl}$**(Warsaw-down)** | | | | | | | | |
|---|---|---|---|---|---|---|---|---|
| $ijkl$ | $\lvert P_a^{sb}\rvert$ | $\arg(P_a^{sb})$ | $\lvert P_a^{db}\rvert$ | $\arg(P_a^{db})$ | $\lvert P_a^{sd}\rvert$ | $\arg(P_a^{sd})$ | $\lvert P_a^{cu}\rvert$ | $\arg(P_a^{cu})$ |
| 1111 | - | - | $(7.77)10^{-4}$ | 44 | - | - | - | - |
| 1112 | $(1.45)10^{-4}$ | -157 | $(3.61)10^{-3}$ | -159 | 0.03 | -157 | - | - |
| 1113 | $(2.75)10^{-4}$ | 178 | 0.27 | 22 | $(4.80)10^{-4}$ | 24 | - | - |
| 1122 | $(6.68)10^{-4}$ | -2 | - | - | - | - | - | - |
| 1123 | 0.05 | 179 | $(1.51)10^{-3}$ | 44 | - | - | - | - |
| 1133 | 0.02 | 178 | 0.02 | -136 | $(1.18)10^{-4}$ | -134 | - | - |
| 2211 | - | - | $(7.77)10^{-4}$ | 44 | - | - | - | - |
| 2212 | $(1.45)10^{-4}$ | -157 | $(3.61)10^{-3}$ | -159 | 0.03 | -157 | - | - |
| 2213 | $(2.75)10^{-4}$ | 178 | 0.27 | 22 | $(4.80)10^{-4}$ | 24 | - | - |
| 2222 | $(6.68)10^{-4}$ | -2 | - | - | - | - | - | - |
| 2223 | 0.05 | 179 | $(1.51)10^{-3}$ | 44 | - | - | - | - |
| 2233 | 0.02 | 178 | 0.02 | -136 | $(1.18)10^{-4}$ | -134 | - | - |
| 3311 | - | - | $(7.64)10^{-4}$ | 44 | - | - | - | - |
| 3312 | $(1.56)10^{-4}$ | -159 | $(3.63)10^{-3}$ | -159 | 0.03 | -157 | - | - |
| 3313 | - | - | 0.27 | 22 | $(4.82)10^{-4}$ | 24 | - | - |
| 3322 | $(6.85)10^{-4}$ | -2 | - | - | - | - | - | - |
| 3323 | 0.05 | 179 | - | - | $(1.05)10^{-4}$ | -135 | - | - |
| 3333 | $(5.68)10^{-4}$ | -2 | $(6.34)10^{-4}$ | 44 | - | - | - | - |

Table 29: The modulus (in the units of $\text{TeV}^2$) and the argument (in degrees) of $P_a^{ij}(\Lambda)$ in Warsaw-down basis for meson systems at scale $\Lambda = 5\,\text{TeV}$ is shown.

| $[\mathcal{C}_{lq}^{(3)}]_{ijkl}$(Warsaw-up) | | | | | | | | |
|---|---|---|---|---|---|---|---|---|
| $ijkl$ | $\lvert P_a^{sb}\rvert$ | $\arg(P_a^{sb})$ | $\lvert P_a^{db}\rvert$ | $\arg(P_a^{db})$ | $\lvert P_a^{sd}\rvert$ | $\arg(P_a^{sd})$ | $\lvert P_a^{cu}\rvert$ | $\arg(P_a^{cu})$ |
| 1111 | - | - | $(6.49)10^{-4}$ | -52 | $(6.62)10^{-3}$ | -157 | - | - |
| 1112 | $(3.98)10^{-4}$ | 161 | $(7.51)10^{-3}$ | 23 | 0.03 | -157 | - | - |
| 1113 | 0.01 | 179 | 0.26 | 22 | $(1.61)10^{-3}$ | 23 | - | - |
| 1122 | $(1.50)10^{-3}$ | 179 | $(1.75)10^{-3}$ | -158 | $(6.61)10^{-3}$ | 23 | - | - |
| 1123 | 0.05 | 179 | 0.06 | -158 | $(7.47)10^{-4}$ | -146 | - | - |
| 1133 | 0.01 | 178 | 0.02 | -136 | - | - | - | - |
| 2211 | - | - | $(6.49)10^{-4}$ | -52 | $(6.62)10^{-3}$ | -157 | - | - |
| 2212 | $(3.98)10^{-4}$ | 161 | $(7.51)10^{-3}$ | 23 | 0.03 | -157 | - | - |
| 2213 | 0.01 | 179 | 0.26 | 22 | $(1.61)10^{-3}$ | 23 | - | - |
| 2222 | $(1.50)10^{-3}$ | 179 | $(1.75)10^{-3}$ | -158 | $(6.61)10^{-3}$ | 23 | - | - |
| 2223 | 0.05 | 179 | 0.06 | -158 | $(7.47)10^{-4}$ | -146 | - | - |
| 2233 | 0.01 | 178 | 0.02 | -136 | - | - | - | - |
| 3311 | - | - | $(6.50)10^{-4}$ | -54 | $(6.61)10^{-3}$ | -157 | - | - |
| 3312 | $(3.97)10^{-4}$ | 161 | $(7.49)10^{-3}$ | 23 | 0.03 | -157 | - | - |
| 3313 | 0.01 | 179 | 0.26 | 22 | $(1.61)10^{-3}$ | 23 | - | - |
| 3322 | $(1.51)10^{-3}$ | 179 | $(1.76)10^{-3}$ | -158 | $(6.60)10^{-3}$ | 23 | - | - |
| 3323 | 0.05 | 179 | 0.06 | -158 | $(7.47)10^{-4}$ | -146 | - | - |
| 3333 | $(2.77)10^{-3}$ | -2 | $(3.09)10^{-3}$ | 44 | - | - | - | - |

Table 30: The modulus (in the units of $\mathrm{TeV}^2$) and the argument (in degrees) of $P_a^{ij}(\Lambda)$ in Warsaw-up basis for meson systems at scale $\Lambda = 5\,\mathrm{TeV}$ is shown.

| $[\mathcal{C}_{ld}]_{ijkl}$(Warsaw-down) | | | | | | | | |
|---|---|---|---|---|---|---|---|---|
| $ijkl$ | $\lvert P_a^{sb}\rvert$ | $\arg(P_a^{sb})$ | $\lvert P_a^{db}\rvert$ | $\arg(P_a^{db})$ | $\lvert P_a^{sd}\rvert$ | $\arg(P_a^{sd})$ | $\lvert P_a^{cu}\rvert$ | $\arg(P_a^{cu})$ |
| 1112 | - | - | - | - | 0.12 | 22 | - | - |
| 1113 | - | - | 0.02 | -158 | - | - | - | - |
| 1123 | $(4.43)10^{-3}$ | -1 | - | - | - | - | - | - |
| 2212 | - | - | - | - | 0.12 | 22 | - | - |
| 2213 | - | - | 0.02 | -158 | - | - | - | - |
| 2223 | $(4.43)10^{-3}$ | -1 | - | - | - | - | - | - |
| 3312 | - | - | - | - | 0.12 | 22 | - | - |
| 3313 | - | - | 0.02 | -158 | - | - | - | - |
| 3323 | $(4.50)10^{-3}$ | -1 | - | - | - | - | - | - |

Table 31: The modulus (in the units of $\mathrm{TeV}^2$) and the argument (in degrees) of $P_a^{ij}(\Lambda)$ in Warsaw-down basis for meson systems at scale $\Lambda = 5\,\mathrm{TeV}$ is shown.

| $[\mathcal{C}_{ld}]_{ijkl}$**(Warsaw-up)** | | | | | | | | |
|---|---|---|---|---|---|---|---|---|
| $ijkl$ | $\lvert P_a^{sb}\rvert$ | $\arg(P_a^{sb})$ | $\lvert P_a^{db}\rvert$ | $\arg(P_a^{db})$ | $\lvert P_a^{ds}\rvert$ | $\arg(P_a^{ds})$ | $\lvert P_a^{uc}\rvert$ | $\arg(P_a^{uc})$ |
| 1112 | - | - | - | - | 0.12 | 22 | - | - |
| 1113 | - | - | 0.02 | -158 | - | - | - | - |
| 1123 | $(4.43)10^{-3}$ | -1 | - | - | - | - | - | - |
| 2212 | - | - | - | - | 0.12 | 22 | - | - |
| 2213 | - | - | 0.02 | -158 | - | - | - | - |
| 2223 | $(4.43)10^{-3}$ | -1 | - | - | - | - | - | - |
| 3312 | - | - | - | - | 0.12 | 22 | - | - |
| 3313 | - | - | 0.02 | -158 | - | - | - | - |
| 3323 | $(4.50)10^{-3}$ | -1 | - | - | - | - | - | - |

Table 32: The modulus (in the units of $\text{TeV}^2$) and the argument (in degrees) of $P_a^{ij}(\Lambda)$ in Warsaw-up basis for meson systems at scale $\Lambda = 5\,\text{TeV}$ is shown.

| $[\mathcal{C}_{qe}]_{ijkl}$**(Warsaw-down)** | | | | | | | | |
|---|---|---|---|---|---|---|---|---|
| $ijkl$ | $\lvert P_a^{sb}\rvert$ | $\arg(P_a^{sb})$ | $\lvert P_a^{db}\rvert$ | $\arg(P_a^{db})$ | $\lvert P_a^{sd}\rvert$ | $\arg(P_a^{sd})$ | $\lvert P_a^{cu}\rvert$ | $\arg(P_a^{cu})$ |
| 1211 | - | - | - | - | $(2.95)10^{-4}$ | 22 | - | - |
| 1222 | - | - | - | - | $(2.95)10^{-4}$ | 22 | - | - |
| 1233 | - | - | - | - | $(3.07)10^{-4}$ | 22 | - | - |
| 1311 | - | - | $(2.90)10^{-3}$ | -158 | - | - | - | - |
| 1322 | - | - | $(2.90)10^{-3}$ | -158 | - | - | - | - |
| 1333 | - | - | $(2.97)10^{-3}$ | -158 | - | - | - | - |
| 2311 | $(5.71)10^{-4}$ | -1 | - | - | - | - | - | - |
| 2322 | $(5.71)10^{-4}$ | -1 | - | - | - | - | - | - |
| 2333 | $(5.85)10^{-4}$ | -1 | - | - | - | - | - | - |

Table 33: The modulus (in the units of $\text{TeV}^2$) and the argument (in degrees) of $P_a^{ij}(\Lambda)$ in Warsaw-down basis for meson systems at scale $\Lambda = 5\,\text{TeV}$ is shown.

| $[\mathcal{C}_{qe}]_{ijkl}$**(Warsaw-up)** | | | | | | | | |
|---|---|---|---|---|---|---|---|---|
| $ijkl$ | $\lvert P_a^{sb}\rvert$ | $\arg(P_a^{sb})$ | $\lvert P_a^{db}\rvert$ | $\arg(P_a^{db})$ | $\lvert P_a^{sd}\rvert$ | $\arg(P_a^{sd})$ | $\lvert P_a^{cu}\rvert$ | $\arg(P_a^{cu})$ |
| 1211 | - | - | - | - | $(2.65)10^{-4}$ | 22 | - | - |
| 1222 | - | - | - | - | $(2.65)10^{-4}$ | 22 | - | - |
| 1233 | - | - | - | - | $(2.76)10^{-4}$ | 22 | - | - |
| 1311 | $(1.28)10^{-4}$ | -1 | $(2.83)10^{-3}$ | -158 | - | - | - | - |
| 1322 | $(1.28)10^{-4}$ | -1 | $(2.83)10^{-3}$ | -158 | - | - | - | - |
| 1333 | $(1.31)10^{-4}$ | -1 | $(2.90)10^{-3}$ | -158 | - | - | - | - |
| 2311 | $(5.55)10^{-4}$ | -1 | $(6.50)10^{-4}$ | 22 | - | - | - | - |
| 2322 | $(5.55)10^{-4}$ | -1 | $(6.50)10^{-4}$ | 22 | - | - | - | - |
| 2333 | $(5.69)10^{-4}$ | -1 | $(6.66)10^{-4}$ | 22 | - | - | - | - |

Table 34: The modulus (in the units of $\text{TeV}^2$) and the argument (in degrees) of $P_a^{ij}(\Lambda)$ in Warsaw-up basis for meson systems at scale $\Lambda = 5\,\text{TeV}$ is shown.
